# Supplementary material for: Blind Image Restoration with Flow Based Priors
Source: arXiv:2009.04583 source file (2020-09-09)
Supplement: Supplementary file 1 [file layers.tex]

\section{Normalizing Flow Layers}

In this section we describe all layers that were used in our method's normalizing flow. All layers must fulfill two requirements. First, a layer needs to be easily invertible. Second, a layer need to have an easy to compute determinate. 

\subsection{Affine Coupling Layers}
Affine Coupling Layers were introduced in \cite{RealNVP}. Given some input $x$ it is first split into two disjoint parts $x_1$ and $x_2$. These two parts are then transformed as
\begin{align}
y_1 &= x_1 \\
y_2 &= x_2 \odot s(x_1) + t(x_1)
\end{align}
where the final output $y$ is the concatenation of $y_1$ and $y_2$. $s$ and $t$ are arbitrary functions that compute scale and translation from $x_1$. In order for this process to be invertible one needs to ensure that $\forall x \ s(x) \neq 0$. In practice this can be achieved easily by applying an exponential to the output of $s$. That is using $exp(s(x_1))$ as the scale.

The inverse is computed as
\begin{align}
x_1 &= y_1 \\
x_2 &= \frac{y_2 - t(x_1)}{s(x_1)}
\end{align}

Finally, the jacobian determinant's logarithm of this transformation can be computed as follows:
\begin{align}
\det(\frac{\partial y}{\partial x}) 
&= \det \left[ \begin{matrix} \frac{\partial y_1}{\partial x_1} & \frac{\partial y_1}{\partial x_2} \\ \frac{\partial y_2}{\partial x_1} & \frac{\partial y_2}{\partial x_2} \end{matrix} \right] \\
&= \det \left[ \begin{matrix} I & 0 \\ \frac{\partial y_2}{\partial x_1} & diag(s(x_1)) \end{matrix} \right] \\
&= \det (I) \cdot \det (diag(s(x_1))) \\
&= \prod{s(x_1)} \\
\Rightarrow \log \det(\frac{\partial y}{\partial x}) &= \sum{ \log s(x_1)}
\end{align}

\subsection{One by One Convolution}
\label{sec:one_by_one_conv}
Convolutional layers are widely used in deep neural networks. As standard convolutions are not invertible \cite{Glow} introduced invertible one by one convolutions to be used in normalizing flows. As the name suggests one by one convolutions use a filter of size 1x1. In order for the convolution to be invertible the weight matrix $W$ needs to be invertible. The convolution as well as its inverse are trivial to compute using $W$ and its inverse $W^{-1}$. 

As a consequence of the filter size being 1x1 spacial dimensions are independent of each other. Due to this the jacobian's determinant is simple to compute as $\left | \det W \right | ^ {h \cdot w}$, where $h$ and $w$ are the input's height and width. The jacobian determinant's logarithm can then be computed as $h \cdot w \cdot \left | \det W \right |$.

\subsection{Actnorm}
Actnorm layers were introduced in \cite{Glow} as an alternative to batch normalization when using small batch sizes. Actnorm layers contain a translation $t$ and scale $s$ parameter for each input channel. Given single channel input $x$ the output $y$ is computed as $y = s*x + t$. The inverse is trivial to compute as $x = \frac{y-t}{s}$. In order for the inverse to be well defined one must ensure that $s > 0$ holds. Similar to the Affine Coupling Layer this can be achieved by using an exponential. Should the input contain multiple channels each one is treated separately with its own translation and scale parameters. 

The parameters $s$ and $t$ are initialized using the first batch during training. They are initialized in a way such that the output is normalized to the desired range. Common ranges used are $[0, 1]$ and $[-0.5, 0.5]$. After initialization the scale and translation parameters are treated like any other parameter.

The jacobian determinant can be computed as $\prod_{i}{s_i^{h \cdot w}}$, where $s_i$ refers to the scale parameter for the $ith$ channel and $h$, $w$ refer to the input's height and width respectively. The resulting logarithm is $h \cdot w \cdot \sum_i{s_i}$.

\subsection{Squeezing}
Together with the multi-scale architecture \cite{RealNVP} introduced squeezing layers. Squeezing layers perform a simple space-to-depth rearrangement of the input tensor by some factor $f$. The input tensor's spacial dimensions are split into tiles with edge length $f$. All values in a given tile are then stacked along the same channel. This divides the size of each spacial dimension by a factor of $f$ while it increases the number of channels by a factor of $f^D$, where $D$ is the number of spacial dimensions. As this operation is a simple rearrangement of variables inversion is trivial and its jacobian's determinant is equal to one. In our work squeezing layers with factor two are used as the first layer for each level.
