# Supplementary material for: Blind Image Restoration with Flow Based Priors
Source: arXiv:2009.04583 source file (2020-09-09)
Supplement: Supplementary file 2 [file colorbrewer.tex]

\usepackage{pgfplotstable}

% Macro for creating a cycle list from a table.
% Makes it easier to define only as many cycle list entries as
% there are colorbrewer values
\newcommand\pgfplotscreatecolorbrewercyclelist{	\pgfmathtruncatemacro\maxindex{\pgfkeysvalueof{/pgfplots/colorbrewer values}-1}
	\pgfplotstabletypeset[
		begin table={},
		end table={},
		skip coltypes,
		string type,
		col sep=semicolon,
		write to macro=\listmacro,
		skip rows between index={\maxindex}{99},
		typeset=false,
		row sep=crcr
	]{
	colorbrewer1, thick, mark=*\\
	colorbrewer2, thick, mark=square*, mark size=1.75\\
	colorbrewer3, thick, mark=triangle*, mark size=2.5\\
	colorbrewer4, thick, mark=x, mark size=3, mark options={line width=2\pgflinewidth}\\
	colorbrewer5, thick, mark=*, mark options={fill=white}\\
	colorbrewer6, thick, mark=square*, mark size=1.75, mark options={fill=white}\\
	colorbrewer7, thick, mark=triangle*, mark size=2.5, mark options={fill=white}\\
	colorbrewer8, thick, mark=+, mark size=3, mark options={line width=2\pgflinewidth}\\
	}
	\begingroup
    \edef\A{\noexpand\global\noexpand\pgfplotscreateplotcyclelist{colorbrewer}{\unexpanded\expandafter{\listmacro}}}%
    \expandafter
    \endgroup\A
}

\pgfplotsset{
	colorbrewer values/.initial=8,
	colorbrewer scheme/.code={
		\pgfplotsset{colorbrewer scheme/#1}
		\pgfplotsset{colorbrewer values/\pgfkeysvalueof{/pgfplots/colorbrewer values}}
	},
	colorbrewer cycle list/.style={
		colorbrewer create cycle list,
		cycle list name=colorbrewer,
		/pgfplots/execute at begin axis={
			\pgfplotsset{
				colorbrewer scheme/#1,
				colorbrewer values/\pgfkeysvalueof{/pgfplots/colorbrewer values}
			}
		}
	},
	colorbrewer cycle list/.default=Dark2,
	colorbrewer create cycle list/.code={
		\pgfplotscreatecolorbrewercyclelist
	}
}

%%% The color schemes

\pgfplotsset{
	colorbrewer scheme/.is choice, 
	colorbrewer scheme/Accent/.style={
		colorbrewer values/.is choice,
		colorbrewer values/3/.code={
			\definecolor{colorbrewer1}{RGB}{127,201,127}
			\definecolor{colorbrewer2}{RGB}{190,174,212}
			\definecolor{colorbrewer3}{RGB}{253,192,134}
		},
		colorbrewer values=3,
		colorbrewer values/4/.code={
			\definecolor{colorbrewer1}{RGB}{127,201,127}
			\definecolor{colorbrewer2}{RGB}{190,174,212}
			\definecolor{colorbrewer3}{RGB}{253,192,134}
			\definecolor{colorbrewer4}{RGB}{255,255,153}
		},
		colorbrewer values/5/.code={
			\definecolor{colorbrewer1}{RGB}{127,201,127}
			\definecolor{colorbrewer2}{RGB}{190,174,212}
			\definecolor{colorbrewer3}{RGB}{253,192,134}
			\definecolor{colorbrewer4}{RGB}{255,255,153}
			\definecolor{colorbrewer5}{RGB}{56,108,176}
		},
		colorbrewer values/6/.code={
			\definecolor{colorbrewer1}{RGB}{127,201,127}
			\definecolor{colorbrewer2}{RGB}{190,174,212}
			\definecolor{colorbrewer3}{RGB}{253,192,134}
			\definecolor{colorbrewer4}{RGB}{255,255,153}
			\definecolor{colorbrewer5}{RGB}{56,108,176}
			\definecolor{colorbrewer6}{RGB}{240,2,127}
		},
		colorbrewer values/7/.code={
			\definecolor{colorbrewer1}{RGB}{127,201,127}
			\definecolor{colorbrewer2}{RGB}{190,174,212}
			\definecolor{colorbrewer3}{RGB}{253,192,134}
			\definecolor{colorbrewer4}{RGB}{255,255,153}
			\definecolor{colorbrewer5}{RGB}{56,108,176}
			\definecolor{colorbrewer6}{RGB}{240,2,127}
			\definecolor{colorbrewer7}{RGB}{191,91,23}
		},
		colorbrewer values/8/.code={
			\definecolor{colorbrewer1}{RGB}{127,201,127}
			\definecolor{colorbrewer2}{RGB}{190,174,212}
			\definecolor{colorbrewer3}{RGB}{253,192,134}
			\definecolor{colorbrewer4}{RGB}{255,255,153}
			\definecolor{colorbrewer5}{RGB}{56,108,176}
			\definecolor{colorbrewer6}{RGB}{240,2,127}
			\definecolor{colorbrewer7}{RGB}{191,91,23}
			\definecolor{colorbrewer8}{RGB}{102,102,102}
		},
		colorbrewer values/.unknown/.style={/errors/unknown choice value=\pgfkeyscurrentkey\pgfkeyscurrentvalue}
	},
	colorbrewer scheme/Blues/.style={
		colorbrewer values/.is choice,	
		colorbrewer values/3/.code={
			\definecolor{colorbrewer1}{RGB}{222,235,247}
			\definecolor{colorbrewer2}{RGB}{158,202,225}
			\definecolor{colorbrewer3}{RGB}{49,130,189}
		},
		colorbrewer values=3,
		colorbrewer values/4/.code={
			\definecolor{colorbrewer1}{RGB}{239,243,255}
			\definecolor{colorbrewer2}{RGB}{189,215,231}
			\definecolor{colorbrewer3}{RGB}{107,174,214}
			\definecolor{colorbrewer4}{RGB}{33,113,181}
		},
		colorbrewer values/5/.code={
			\definecolor{colorbrewer1}{RGB}{239,243,255}
			\definecolor{colorbrewer2}{RGB}{189,215,231}
			\definecolor{colorbrewer3}{RGB}{107,174,214}
			\definecolor{colorbrewer4}{RGB}{49,130,189}
			\definecolor{colorbrewer5}{RGB}{8,81,156}
		},
		colorbrewer values/6/.code={
			\definecolor{colorbrewer1}{RGB}{239,243,255}
			\definecolor{colorbrewer2}{RGB}{198,219,239}
			\definecolor{colorbrewer3}{RGB}{158,202,225}
			\definecolor{colorbrewer4}{RGB}{107,174,214}
			\definecolor{colorbrewer5}{RGB}{49,130,189}
			\definecolor{colorbrewer6}{RGB}{8,81,156}
		},
		colorbrewer values/7/.code={
			\definecolor{colorbrewer1}{RGB}{239,243,255}
			\definecolor{colorbrewer2}{RGB}{198,219,239}
			\definecolor{colorbrewer3}{RGB}{158,202,225}
			\definecolor{colorbrewer4}{RGB}{107,174,214}
			\definecolor{colorbrewer5}{RGB}{66,146,198}
			\definecolor{colorbrewer6}{RGB}{33,113,181}
			\definecolor{colorbrewer7}{RGB}{8,69,148}
		},
		colorbrewer values/8/.code={
			\definecolor{colorbrewer1}{RGB}{247,251,255}
			\definecolor{colorbrewer2}{RGB}{222,235,247}
			\definecolor{colorbrewer3}{RGB}{198,219,239}
			\definecolor{colorbrewer4}{RGB}{158,202,225}
			\definecolor{colorbrewer5}{RGB}{107,174,214}
			\definecolor{colorbrewer6}{RGB}{66,146,198}
			\definecolor{colorbrewer7}{RGB}{33,113,181}
			\definecolor{colorbrewer8}{RGB}{8,69,148}
		},
		colorbrewer values/9/.code={
			\definecolor{colorbrewer1}{RGB}{247,251,255}
			\definecolor{colorbrewer2}{RGB}{222,235,247}
			\definecolor{colorbrewer3}{RGB}{198,219,239}
			\definecolor{colorbrewer4}{RGB}{158,202,225}
			\definecolor{colorbrewer5}{RGB}{107,174,214}
			\definecolor{colorbrewer6}{RGB}{66,146,198}
			\definecolor{colorbrewer7}{RGB}{33,113,181}
			\definecolor{colorbrewer8}{RGB}{8,81,156}
			\definecolor{colorbrewer9}{RGB}{8,48,107}
		}
	},
	colorbrewer scheme/BrBG/.style={
		colorbrewer values/.is choice,	
		colorbrewer values/3/.code={
			\definecolor{colorbrewer1}{RGB}{216,179,101}
			\definecolor{colorbrewer2}{RGB}{245,245,245}
			\definecolor{colorbrewer3}{RGB}{90,180,172}
		},
		colorbrewer values=3,
		colorbrewer values/4/.code={
			\definecolor{colorbrewer1}{RGB}{166,97,26}
			\definecolor{colorbrewer2}{RGB}{223,194,125}
			\definecolor{colorbrewer3}{RGB}{128,205,193}
			\definecolor{colorbrewer4}{RGB}{1,133,113}
		},
		colorbrewer values/5/.code={
			\definecolor{colorbrewer1}{RGB}{166,97,26}
			\definecolor{colorbrewer2}{RGB}{223,194,125}
			\definecolor{colorbrewer3}{RGB}{245,245,245}
			\definecolor{colorbrewer4}{RGB}{128,205,193}
			\definecolor{colorbrewer5}{RGB}{1,133,113}
		},
		colorbrewer values/6/.code={
			\definecolor{colorbrewer1}{RGB}{140,81,10}
			\definecolor{colorbrewer2}{RGB}{216,179,101}
			\definecolor{colorbrewer3}{RGB}{246,232,195}
			\definecolor{colorbrewer4}{RGB}{199,234,229}
			\definecolor{colorbrewer5}{RGB}{90,180,172}
			\definecolor{colorbrewer6}{RGB}{1,102,94}
		},
		colorbrewer values/7/.code={
			\definecolor{colorbrewer1}{RGB}{140,81,10}
			\definecolor{colorbrewer2}{RGB}{216,179,101}
			\definecolor{colorbrewer3}{RGB}{246,232,195}
			\definecolor{colorbrewer4}{RGB}{245,245,245}
			\definecolor{colorbrewer5}{RGB}{199,234,229}
			\definecolor{colorbrewer6}{RGB}{90,180,172}
			\definecolor{colorbrewer7}{RGB}{1,102,94}
		},
		colorbrewer values/8/.code={
			\definecolor{colorbrewer1}{RGB}{140,81,10}
			\definecolor{colorbrewer2}{RGB}{191,129,45}
			\definecolor{colorbrewer3}{RGB}{223,194,125}
			\definecolor{colorbrewer4}{RGB}{246,232,195}
			\definecolor{colorbrewer5}{RGB}{199,234,229}
			\definecolor{colorbrewer6}{RGB}{128,205,193}
			\definecolor{colorbrewer7}{RGB}{53,151,143}
			\definecolor{colorbrewer8}{RGB}{1,102,94}
		},
		colorbrewer values/9/.code={
			\definecolor{colorbrewer1}{RGB}{140,81,10}
			\definecolor{colorbrewer2}{RGB}{191,129,45}
			\definecolor{colorbrewer3}{RGB}{223,194,125}
			\definecolor{colorbrewer4}{RGB}{246,232,195}
			\definecolor{colorbrewer5}{RGB}{245,245,245}
			\definecolor{colorbrewer6}{RGB}{199,234,229}
			\definecolor{colorbrewer7}{RGB}{128,205,193}
			\definecolor{colorbrewer8}{RGB}{53,151,143}
			\definecolor{colorbrewer9}{RGB}{1,102,94}
		},
		colorbrewer values/10/.code={
			\definecolor{colorbrewer1}{RGB}{84,48,5}
			\definecolor{colorbrewer2}{RGB}{140,81,10}
			\definecolor{colorbrewer3}{RGB}{191,129,45}
			\definecolor{colorbrewer4}{RGB}{223,194,125}
			\definecolor{colorbrewer5}{RGB}{246,232,195}
			\definecolor{colorbrewer6}{RGB}{199,234,229}
			\definecolor{colorbrewer7}{RGB}{128,205,193}
			\definecolor{colorbrewer8}{RGB}{53,151,143}
			\definecolor{colorbrewer9}{RGB}{1,102,94}
			\definecolor{colorbrewer10}{RGB}{0,60,48}
		},
		colorbrewer values/11/.code={
			\definecolor{colorbrewer1}{RGB}{84,48,5}
			\definecolor{colorbrewer2}{RGB}{140,81,10}
			\definecolor{colorbrewer3}{RGB}{191,129,45}
			\definecolor{colorbrewer4}{RGB}{223,194,125}
			\definecolor{colorbrewer5}{RGB}{246,232,195}
			\definecolor{colorbrewer6}{RGB}{245,245,245}
			\definecolor{colorbrewer7}{RGB}{199,234,229}
			\definecolor{colorbrewer8}{RGB}{128,205,193}
			\definecolor{colorbrewer9}{RGB}{53,151,143}
			\definecolor{colorbrewer10}{RGB}{1,102,94}
			\definecolor{colorbrewer11}{RGB}{0,60,48}
		}
	},
	colorbrewer scheme/BuGn/.style={
		colorbrewer values/.is choice,	
		colorbrewer values/3/.code={
			\definecolor{colorbrewer1}{RGB}{229,245,249}
			\definecolor{colorbrewer2}{RGB}{153,216,201}
			\definecolor{colorbrewer3}{RGB}{44,162,95}
		},
		colorbrewer values=3,
		colorbrewer values/4/.code={
			\definecolor{colorbrewer1}{RGB}{237,248,251}
			\definecolor{colorbrewer2}{RGB}{178,226,226}
			\definecolor{colorbrewer3}{RGB}{102,194,164}
			\definecolor{colorbrewer4}{RGB}{35,139,69}
		},
		colorbrewer values/5/.code={
			\definecolor{colorbrewer1}{RGB}{237,248,251}
			\definecolor{colorbrewer2}{RGB}{178,226,226}
			\definecolor{colorbrewer3}{RGB}{102,194,164}
			\definecolor{colorbrewer4}{RGB}{44,162,95}
			\definecolor{colorbrewer5}{RGB}{0,109,44}
		},
		colorbrewer values/6/.code={
			\definecolor{colorbrewer1}{RGB}{237,248,251}
			\definecolor{colorbrewer2}{RGB}{204,236,230}
			\definecolor{colorbrewer3}{RGB}{153,216,201}
			\definecolor{colorbrewer4}{RGB}{102,194,164}
			\definecolor{colorbrewer5}{RGB}{44,162,95}
			\definecolor{colorbrewer6}{RGB}{0,109,44}
		},
		colorbrewer values/7/.code={
			\definecolor{colorbrewer1}{RGB}{237,248,251}
			\definecolor{colorbrewer2}{RGB}{204,236,230}
			\definecolor{colorbrewer3}{RGB}{153,216,201}
			\definecolor{colorbrewer4}{RGB}{102,194,164}
			\definecolor{colorbrewer5}{RGB}{65,174,118}
			\definecolor{colorbrewer6}{RGB}{35,139,69}
			\definecolor{colorbrewer7}{RGB}{0,88,36}
		},
		colorbrewer values/8/.code={
			\definecolor{colorbrewer1}{RGB}{247,252,253}
			\definecolor{colorbrewer2}{RGB}{229,245,249}
			\definecolor{colorbrewer3}{RGB}{204,236,230}
			\definecolor{colorbrewer4}{RGB}{153,216,201}
			\definecolor{colorbrewer5}{RGB}{102,194,164}
			\definecolor{colorbrewer6}{RGB}{65,174,118}
			\definecolor{colorbrewer7}{RGB}{35,139,69}
			\definecolor{colorbrewer8}{RGB}{0,88,36}
		},
		colorbrewer values/9/.code={
			\definecolor{colorbrewer1}{RGB}{247,252,253}
			\definecolor{colorbrewer2}{RGB}{229,245,249}
			\definecolor{colorbrewer3}{RGB}{204,236,230}
			\definecolor{colorbrewer4}{RGB}{153,216,201}
			\definecolor{colorbrewer5}{RGB}{102,194,164}
			\definecolor{colorbrewer6}{RGB}{65,174,118}
			\definecolor{colorbrewer7}{RGB}{35,139,69}
			\definecolor{colorbrewer8}{RGB}{0,109,44}
			\definecolor{colorbrewer9}{RGB}{0,68,27}
		}
	},
	colorbrewer scheme/BuPu/.style={
		colorbrewer values/.is choice,	
		colorbrewer values/3/.code={
			\definecolor{colorbrewer1}{RGB}{224,236,244}
			\definecolor{colorbrewer2}{RGB}{158,188,218}
			\definecolor{colorbrewer3}{RGB}{136,86,167}
		},
		colorbrewer values=3,
		colorbrewer values/4/.code={
			\definecolor{colorbrewer1}{RGB}{237,248,251}
			\definecolor{colorbrewer2}{RGB}{179,205,227}
			\definecolor{colorbrewer3}{RGB}{140,150,198}
			\definecolor{colorbrewer4}{RGB}{136,65,157}
		},
		colorbrewer values/5/.code={
			\definecolor{colorbrewer1}{RGB}{237,248,251}
			\definecolor{colorbrewer2}{RGB}{179,205,227}
			\definecolor{colorbrewer3}{RGB}{140,150,198}
			\definecolor{colorbrewer4}{RGB}{136,86,167}
			\definecolor{colorbrewer5}{RGB}{129,15,124}
		},
		colorbrewer values/6/.code={
			\definecolor{colorbrewer1}{RGB}{237,248,251}
			\definecolor{colorbrewer2}{RGB}{191,211,230}
			\definecolor{colorbrewer3}{RGB}{158,188,218}
			\definecolor{colorbrewer4}{RGB}{140,150,198}
			\definecolor{colorbrewer5}{RGB}{136,86,167}
			\definecolor{colorbrewer6}{RGB}{129,15,124}
		},
		colorbrewer values/7/.code={
			\definecolor{colorbrewer1}{RGB}{237,248,251}
			\definecolor{colorbrewer2}{RGB}{191,211,230}
			\definecolor{colorbrewer3}{RGB}{158,188,218}
			\definecolor{colorbrewer4}{RGB}{140,150,198}
			\definecolor{colorbrewer5}{RGB}{140,107,177}
			\definecolor{colorbrewer6}{RGB}{136,65,157}
			\definecolor{colorbrewer7}{RGB}{110,1,107}
		},
		colorbrewer values/8/.code={
			\definecolor{colorbrewer1}{RGB}{247,252,253}
			\definecolor{colorbrewer2}{RGB}{224,236,244}
			\definecolor{colorbrewer3}{RGB}{191,211,230}
			\definecolor{colorbrewer4}{RGB}{158,188,218}
			\definecolor{colorbrewer5}{RGB}{140,150,198}
			\definecolor{colorbrewer6}{RGB}{140,107,177}
			\definecolor{colorbrewer7}{RGB}{136,65,157}
			\definecolor{colorbrewer8}{RGB}{110,1,107}
		},
		colorbrewer values/9/.code={
			\definecolor{colorbrewer1}{RGB}{247,252,253}
			\definecolor{colorbrewer2}{RGB}{224,236,244}
			\definecolor{colorbrewer3}{RGB}{191,211,230}
			\definecolor{colorbrewer4}{RGB}{158,188,218}
			\definecolor{colorbrewer5}{RGB}{140,150,198}
			\definecolor{colorbrewer6}{RGB}{140,107,177}
			\definecolor{colorbrewer7}{RGB}{136,65,157}
			\definecolor{colorbrewer8}{RGB}{129,15,124}
			\definecolor{colorbrewer9}{RGB}{77,0,75}
		}
	},
	colorbrewer scheme/Dark2/.style={
		colorbrewer values/.is choice,	
		colorbrewer values/3/.code={
			\definecolor{colorbrewer1}{RGB}{27,158,119}
			\definecolor{colorbrewer2}{RGB}{217,95,2}
			\definecolor{colorbrewer3}{RGB}{117,112,179}
		},
		colorbrewer values=3,
		colorbrewer values/4/.code={
			\definecolor{colorbrewer1}{RGB}{27,158,119}
			\definecolor{colorbrewer2}{RGB}{217,95,2}
			\definecolor{colorbrewer3}{RGB}{117,112,179}
			\definecolor{colorbrewer4}{RGB}{231,41,138}
		},
		colorbrewer values/5/.code={
			\definecolor{colorbrewer1}{RGB}{27,158,119}
			\definecolor{colorbrewer2}{RGB}{217,95,2}
			\definecolor{colorbrewer3}{RGB}{117,112,179}
			\definecolor{colorbrewer4}{RGB}{231,41,138}
			\definecolor{colorbrewer5}{RGB}{102,166,30}
		},
		colorbrewer values/6/.code={
			\definecolor{colorbrewer1}{RGB}{27,158,119}
			\definecolor{colorbrewer2}{RGB}{217,95,2}
			\definecolor{colorbrewer3}{RGB}{117,112,179}
			\definecolor{colorbrewer4}{RGB}{231,41,138}
			\definecolor{colorbrewer5}{RGB}{102,166,30}
			\definecolor{colorbrewer6}{RGB}{230,171,2}
		},
		colorbrewer values/7/.code={
			\definecolor{colorbrewer1}{RGB}{27,158,119}
			\definecolor{colorbrewer2}{RGB}{217,95,2}
			\definecolor{colorbrewer3}{RGB}{117,112,179}
			\definecolor{colorbrewer4}{RGB}{231,41,138}
			\definecolor{colorbrewer5}{RGB}{102,166,30}
			\definecolor{colorbrewer6}{RGB}{230,171,2}
			\definecolor{colorbrewer7}{RGB}{166,118,29}
		},
		colorbrewer values/8/.code={
			\definecolor{colorbrewer1}{RGB}{27,158,119}
			\definecolor{colorbrewer2}{RGB}{217,95,2}
			\definecolor{colorbrewer3}{RGB}{117,112,179}
			\definecolor{colorbrewer4}{RGB}{231,41,138}
			\definecolor{colorbrewer5}{RGB}{102,166,30}
			\definecolor{colorbrewer6}{RGB}{230,171,2}
			\definecolor{colorbrewer7}{RGB}{166,118,29}
			\definecolor{colorbrewer8}{RGB}{102,102,102}
		}
	},
	colorbrewer scheme/GnBu/.style={
		colorbrewer values/.is choice,	
		colorbrewer values/3/.code={
			\definecolor{colorbrewer1}{RGB}{224,243,219}
			\definecolor{colorbrewer2}{RGB}{168,221,181}
			\definecolor{colorbrewer3}{RGB}{67,162,202}
		},
		colorbrewer values=3,
		colorbrewer values/4/.code={
			\definecolor{colorbrewer1}{RGB}{240,249,232}
			\definecolor{colorbrewer2}{RGB}{186,228,188}
			\definecolor{colorbrewer3}{RGB}{123,204,196}
			\definecolor{colorbrewer4}{RGB}{43,140,190}
		},
		colorbrewer values/5/.code={
			\definecolor{colorbrewer1}{RGB}{240,249,232}
			\definecolor{colorbrewer2}{RGB}{186,228,188}
			\definecolor{colorbrewer3}{RGB}{123,204,196}
			\definecolor{colorbrewer4}{RGB}{67,162,202}
			\definecolor{colorbrewer5}{RGB}{8,104,172}
		},
		colorbrewer values/6/.code={
			\definecolor{colorbrewer1}{RGB}{240,249,232}
			\definecolor{colorbrewer2}{RGB}{204,235,197}
			\definecolor{colorbrewer3}{RGB}{168,221,181}
			\definecolor{colorbrewer4}{RGB}{123,204,196}
			\definecolor{colorbrewer5}{RGB}{67,162,202}
			\definecolor{colorbrewer6}{RGB}{8,104,172}
		},
		colorbrewer values/7/.code={
			\definecolor{colorbrewer1}{RGB}{240,249,232}
			\definecolor{colorbrewer2}{RGB}{204,235,197}
			\definecolor{colorbrewer3}{RGB}{168,221,181}
			\definecolor{colorbrewer4}{RGB}{123,204,196}
			\definecolor{colorbrewer5}{RGB}{78,179,211}
			\definecolor{colorbrewer6}{RGB}{43,140,190}
			\definecolor{colorbrewer7}{RGB}{8,88,158}
		},
		colorbrewer values/8/.code={
			\definecolor{colorbrewer1}{RGB}{247,252,240}
			\definecolor{colorbrewer2}{RGB}{224,243,219}
			\definecolor{colorbrewer3}{RGB}{204,235,197}
			\definecolor{colorbrewer4}{RGB}{168,221,181}
			\definecolor{colorbrewer5}{RGB}{123,204,196}
			\definecolor{colorbrewer6}{RGB}{78,179,211}
			\definecolor{colorbrewer7}{RGB}{43,140,190}
			\definecolor{colorbrewer8}{RGB}{8,88,158}
		},
		colorbrewer values/9/.code={
			\definecolor{colorbrewer1}{RGB}{247,252,240}
			\definecolor{colorbrewer2}{RGB}{224,243,219}
			\definecolor{colorbrewer3}{RGB}{204,235,197}
			\definecolor{colorbrewer4}{RGB}{168,221,181}
			\definecolor{colorbrewer5}{RGB}{123,204,196}
			\definecolor{colorbrewer6}{RGB}{78,179,211}
			\definecolor{colorbrewer7}{RGB}{43,140,190}
			\definecolor{colorbrewer8}{RGB}{8,104,172}
			\definecolor{colorbrewer9}{RGB}{8,64,129}
		}
	},
	colorbrewer scheme/Greens/.style={
		colorbrewer values/.is choice,	
		colorbrewer values/3/.code={
			\definecolor{colorbrewer1}{RGB}{229,245,224}
			\definecolor{colorbrewer2}{RGB}{161,217,155}
			\definecolor{colorbrewer3}{RGB}{49,163,84}
		},
		colorbrewer values=3,
		colorbrewer values/4/.code={
			\definecolor{colorbrewer1}{RGB}{237,248,233}
			\definecolor{colorbrewer2}{RGB}{186,228,179}
			\definecolor{colorbrewer3}{RGB}{116,196,118}
			\definecolor{colorbrewer4}{RGB}{35,139,69}
		},
		colorbrewer values/5/.code={
			\definecolor{colorbrewer1}{RGB}{237,248,233}
			\definecolor{colorbrewer2}{RGB}{186,228,179}
			\definecolor{colorbrewer3}{RGB}{116,196,118}
			\definecolor{colorbrewer4}{RGB}{49,163,84}
			\definecolor{colorbrewer5}{RGB}{0,109,44}
		},
		colorbrewer values/6/.code={
			\definecolor{colorbrewer1}{RGB}{237,248,233}
			\definecolor{colorbrewer2}{RGB}{199,233,192}
			\definecolor{colorbrewer3}{RGB}{161,217,155}
			\definecolor{colorbrewer4}{RGB}{116,196,118}
			\definecolor{colorbrewer5}{RGB}{49,163,84}
			\definecolor{colorbrewer6}{RGB}{0,109,44}
		},
		colorbrewer values/7/.code={
			\definecolor{colorbrewer1}{RGB}{237,248,233}
			\definecolor{colorbrewer2}{RGB}{199,233,192}
			\definecolor{colorbrewer3}{RGB}{161,217,155}
			\definecolor{colorbrewer4}{RGB}{116,196,118}
			\definecolor{colorbrewer5}{RGB}{65,171,93}
			\definecolor{colorbrewer6}{RGB}{35,139,69}
			\definecolor{colorbrewer7}{RGB}{0,90,50}
		},
		colorbrewer values/8/.code={
			\definecolor{colorbrewer1}{RGB}{247,252,245}
			\definecolor{colorbrewer2}{RGB}{229,245,224}
			\definecolor{colorbrewer3}{RGB}{199,233,192}
			\definecolor{colorbrewer4}{RGB}{161,217,155}
			\definecolor{colorbrewer5}{RGB}{116,196,118}
			\definecolor{colorbrewer6}{RGB}{65,171,93}
			\definecolor{colorbrewer7}{RGB}{35,139,69}
			\definecolor{colorbrewer8}{RGB}{0,90,50}
		},
		colorbrewer values/9/.code={
			\definecolor{colorbrewer1}{RGB}{247,252,245}
			\definecolor{colorbrewer2}{RGB}{229,245,224}
			\definecolor{colorbrewer3}{RGB}{199,233,192}
			\definecolor{colorbrewer4}{RGB}{161,217,155}
			\definecolor{colorbrewer5}{RGB}{116,196,118}
			\definecolor{colorbrewer6}{RGB}{65,171,93}
			\definecolor{colorbrewer7}{RGB}{35,139,69}
			\definecolor{colorbrewer8}{RGB}{0,109,44}
			\definecolor{colorbrewer9}{RGB}{0,68,27}
		}
	},
	colorbrewer scheme/Greys/.style={
		colorbrewer values/.is choice,	
		colorbrewer values/3/.code={
			\definecolor{colorbrewer1}{RGB}{240,240,240}
			\definecolor{colorbrewer2}{RGB}{189,189,189}
			\definecolor{colorbrewer3}{RGB}{99,99,99}
		},
		colorbrewer values=3,
		colorbrewer values/4/.code={
			\definecolor{colorbrewer1}{RGB}{247,247,247}
			\definecolor{colorbrewer2}{RGB}{204,204,204}
			\definecolor{colorbrewer3}{RGB}{150,150,150}
			\definecolor{colorbrewer4}{RGB}{82,82,82}
		},
		colorbrewer values/5/.code={
			\definecolor{colorbrewer1}{RGB}{247,247,247}
			\definecolor{colorbrewer2}{RGB}{204,204,204}
			\definecolor{colorbrewer3}{RGB}{150,150,150}
			\definecolor{colorbrewer4}{RGB}{99,99,99}
			\definecolor{colorbrewer5}{RGB}{37,37,37}
		},
		colorbrewer values/6/.code={
			\definecolor{colorbrewer1}{RGB}{247,247,247}
			\definecolor{colorbrewer2}{RGB}{217,217,217}
			\definecolor{colorbrewer3}{RGB}{189,189,189}
			\definecolor{colorbrewer4}{RGB}{150,150,150}
			\definecolor{colorbrewer5}{RGB}{99,99,99}
			\definecolor{colorbrewer6}{RGB}{37,37,37}
		},
		colorbrewer values/7/.code={
			\definecolor{colorbrewer1}{RGB}{247,247,247}
			\definecolor{colorbrewer2}{RGB}{217,217,217}
			\definecolor{colorbrewer3}{RGB}{189,189,189}
			\definecolor{colorbrewer4}{RGB}{150,150,150}
			\definecolor{colorbrewer5}{RGB}{115,115,115}
			\definecolor{colorbrewer6}{RGB}{82,82,82}
			\definecolor{colorbrewer7}{RGB}{37,37,37}
		},
		colorbrewer values/8/.code={
			\definecolor{colorbrewer1}{RGB}{255,255,255}
			\definecolor{colorbrewer2}{RGB}{240,240,240}
			\definecolor{colorbrewer3}{RGB}{217,217,217}
			\definecolor{colorbrewer4}{RGB}{189,189,189}
			\definecolor{colorbrewer5}{RGB}{150,150,150}
			\definecolor{colorbrewer6}{RGB}{115,115,115}
			\definecolor{colorbrewer7}{RGB}{82,82,82}
			\definecolor{colorbrewer8}{RGB}{37,37,37}
		},
		colorbrewer values/9/.code={
			\definecolor{colorbrewer1}{RGB}{255,255,255}
			\definecolor{colorbrewer2}{RGB}{240,240,240}
			\definecolor{colorbrewer3}{RGB}{217,217,217}
			\definecolor{colorbrewer4}{RGB}{189,189,189}
			\definecolor{colorbrewer5}{RGB}{150,150,150}
			\definecolor{colorbrewer6}{RGB}{115,115,115}
			\definecolor{colorbrewer7}{RGB}{82,82,82}
			\definecolor{colorbrewer8}{RGB}{37,37,37}
			\definecolor{colorbrewer9}{RGB}{0,0,0}
		}
	},
	colorbrewer scheme/Oranges/.style={
		colorbrewer values/.is choice,	
		colorbrewer values/3/.code={
			\definecolor{colorbrewer1}{RGB}{254,230,206}
			\definecolor{colorbrewer2}{RGB}{253,174,107}
			\definecolor{colorbrewer3}{RGB}{230,85,13}
		},
		colorbrewer values=3,
		colorbrewer values/4/.code={
			\definecolor{colorbrewer1}{RGB}{254,237,222}
			\definecolor{colorbrewer2}{RGB}{253,190,133}
			\definecolor{colorbrewer3}{RGB}{253,141,60}
			\definecolor{colorbrewer4}{RGB}{217,71,1}
		},
		colorbrewer values/5/.code={
			\definecolor{colorbrewer1}{RGB}{254,237,222}
			\definecolor{colorbrewer2}{RGB}{253,190,133}
			\definecolor{colorbrewer3}{RGB}{253,141,60}
			\definecolor{colorbrewer4}{RGB}{230,85,13}
			\definecolor{colorbrewer5}{RGB}{166,54,3}
		},
		colorbrewer values/6/.code={
			\definecolor{colorbrewer1}{RGB}{254,237,222}
			\definecolor{colorbrewer2}{RGB}{253,208,162}
			\definecolor{colorbrewer3}{RGB}{253,174,107}
			\definecolor{colorbrewer4}{RGB}{253,141,60}
			\definecolor{colorbrewer5}{RGB}{230,85,13}
			\definecolor{colorbrewer6}{RGB}{166,54,3}
		},
		colorbrewer values/7/.code={
			\definecolor{colorbrewer1}{RGB}{254,237,222}
			\definecolor{colorbrewer2}{RGB}{253,208,162}
			\definecolor{colorbrewer3}{RGB}{253,174,107}
			\definecolor{colorbrewer4}{RGB}{253,141,60}
			\definecolor{colorbrewer5}{RGB}{241,105,19}
			\definecolor{colorbrewer6}{RGB}{217,72,1}
			\definecolor{colorbrewer7}{RGB}{140,45,4}
		},
		colorbrewer values/8/.code={
			\definecolor{colorbrewer1}{RGB}{255,245,235}
			\definecolor{colorbrewer2}{RGB}{254,230,206}
			\definecolor{colorbrewer3}{RGB}{253,208,162}
			\definecolor{colorbrewer4}{RGB}{253,174,107}
			\definecolor{colorbrewer5}{RGB}{253,141,60}
			\definecolor{colorbrewer6}{RGB}{241,105,19}
			\definecolor{colorbrewer7}{RGB}{217,72,1}
			\definecolor{colorbrewer8}{RGB}{140,45,4}
		},
		colorbrewer values/9/.code={
			\definecolor{colorbrewer1}{RGB}{255,245,235}
			\definecolor{colorbrewer2}{RGB}{254,230,206}
			\definecolor{colorbrewer3}{RGB}{253,208,162}
			\definecolor{colorbrewer4}{RGB}{253,174,107}
			\definecolor{colorbrewer5}{RGB}{253,141,60}
			\definecolor{colorbrewer6}{RGB}{241,105,19}
			\definecolor{colorbrewer7}{RGB}{217,72,1}
			\definecolor{colorbrewer8}{RGB}{166,54,3}
			\definecolor{colorbrewer9}{RGB}{127,39,4}
		}
	},
	colorbrewer scheme/OrRd/.style={
		colorbrewer values/.is choice,	
		colorbrewer values/3/.code={
			\definecolor{colorbrewer1}{RGB}{254,232,200}
			\definecolor{colorbrewer2}{RGB}{253,187,132}
			\definecolor{colorbrewer3}{RGB}{227,74,51}
		},
		colorbrewer values=3,
		colorbrewer values/4/.code={
			\definecolor{colorbrewer1}{RGB}{254,240,217}
			\definecolor{colorbrewer2}{RGB}{253,204,138}
			\definecolor{colorbrewer3}{RGB}{252,141,89}
			\definecolor{colorbrewer4}{RGB}{215,48,31}
		},
		colorbrewer values/5/.code={
			\definecolor{colorbrewer1}{RGB}{254,240,217}
			\definecolor{colorbrewer2}{RGB}{253,204,138}
			\definecolor{colorbrewer3}{RGB}{252,141,89}
			\definecolor{colorbrewer4}{RGB}{227,74,51}
			\definecolor{colorbrewer5}{RGB}{179,0,0}
		},
		colorbrewer values/6/.code={
			\definecolor{colorbrewer1}{RGB}{254,240,217}
			\definecolor{colorbrewer2}{RGB}{253,212,158}
			\definecolor{colorbrewer3}{RGB}{253,187,132}
			\definecolor{colorbrewer4}{RGB}{252,141,89}
			\definecolor{colorbrewer5}{RGB}{227,74,51}
			\definecolor{colorbrewer6}{RGB}{179,0,0}
		},
		colorbrewer values/7/.code={
			\definecolor{colorbrewer1}{RGB}{254,240,217}
			\definecolor{colorbrewer2}{RGB}{253,212,158}
			\definecolor{colorbrewer3}{RGB}{253,187,132}
			\definecolor{colorbrewer4}{RGB}{252,141,89}
			\definecolor{colorbrewer5}{RGB}{239,101,72}
			\definecolor{colorbrewer6}{RGB}{215,48,31}
			\definecolor{colorbrewer7}{RGB}{153,0,0}
		},
		colorbrewer values/8/.code={
			\definecolor{colorbrewer1}{RGB}{255,247,236}
			\definecolor{colorbrewer2}{RGB}{254,232,200}
			\definecolor{colorbrewer3}{RGB}{253,212,158}
			\definecolor{colorbrewer4}{RGB}{253,187,132}
			\definecolor{colorbrewer5}{RGB}{252,141,89}
			\definecolor{colorbrewer6}{RGB}{239,101,72}
			\definecolor{colorbrewer7}{RGB}{215,48,31}
			\definecolor{colorbrewer8}{RGB}{153,0,0}
		},
		colorbrewer values/9/.code={
			\definecolor{colorbrewer1}{RGB}{255,247,236}
			\definecolor{colorbrewer2}{RGB}{254,232,200}
			\definecolor{colorbrewer3}{RGB}{253,212,158}
			\definecolor{colorbrewer4}{RGB}{253,187,132}
			\definecolor{colorbrewer5}{RGB}{252,141,89}
			\definecolor{colorbrewer6}{RGB}{239,101,72}
			\definecolor{colorbrewer7}{RGB}{215,48,31}
			\definecolor{colorbrewer8}{RGB}{179,0,0}
			\definecolor{colorbrewer9}{RGB}{127,0,0}
		}
	},
	colorbrewer scheme/Paired/.style={
		colorbrewer values/.is choice,	
		colorbrewer values/3/.code={
			\definecolor{colorbrewer1}{RGB}{166,206,227}
			\definecolor{colorbrewer2}{RGB}{31,120,180}
			\definecolor{colorbrewer3}{RGB}{178,223,138}
		},
		colorbrewer values=3,
		colorbrewer values/4/.code={
			\definecolor{colorbrewer1}{RGB}{166,206,227}
			\definecolor{colorbrewer2}{RGB}{31,120,180}
			\definecolor{colorbrewer3}{RGB}{178,223,138}
			\definecolor{colorbrewer4}{RGB}{51,160,44}
		},
		colorbrewer values/5/.code={
			\definecolor{colorbrewer1}{RGB}{166,206,227}
			\definecolor{colorbrewer2}{RGB}{31,120,180}
			\definecolor{colorbrewer3}{RGB}{178,223,138}
			\definecolor{colorbrewer4}{RGB}{51,160,44}
			\definecolor{colorbrewer5}{RGB}{251,154,153}
		},
		colorbrewer values/6/.code={
			\definecolor{colorbrewer1}{RGB}{166,206,227}
			\definecolor{colorbrewer2}{RGB}{31,120,180}
			\definecolor{colorbrewer3}{RGB}{178,223,138}
			\definecolor{colorbrewer4}{RGB}{51,160,44}
			\definecolor{colorbrewer5}{RGB}{251,154,153}
			\definecolor{colorbrewer6}{RGB}{227,26,28}
		},
		colorbrewer values/7/.code={
			\definecolor{colorbrewer1}{RGB}{166,206,227}
			\definecolor{colorbrewer2}{RGB}{31,120,180}
			\definecolor{colorbrewer3}{RGB}{178,223,138}
			\definecolor{colorbrewer4}{RGB}{51,160,44}
			\definecolor{colorbrewer5}{RGB}{251,154,153}
			\definecolor{colorbrewer6}{RGB}{227,26,28}
			\definecolor{colorbrewer7}{RGB}{253,191,111}
		},
		colorbrewer values/8/.code={
			\definecolor{colorbrewer1}{RGB}{166,206,227}
			\definecolor{colorbrewer2}{RGB}{31,120,180}
			\definecolor{colorbrewer3}{RGB}{178,223,138}
			\definecolor{colorbrewer4}{RGB}{51,160,44}
			\definecolor{colorbrewer5}{RGB}{251,154,153}
			\definecolor{colorbrewer6}{RGB}{227,26,28}
			\definecolor{colorbrewer7}{RGB}{253,191,111}
			\definecolor{colorbrewer8}{RGB}{255,127,0}
		},
		colorbrewer values/9/.code={
			\definecolor{colorbrewer1}{RGB}{166,206,227}
			\definecolor{colorbrewer2}{RGB}{31,120,180}
			\definecolor{colorbrewer3}{RGB}{178,223,138}
			\definecolor{colorbrewer4}{RGB}{51,160,44}
			\definecolor{colorbrewer5}{RGB}{251,154,153}
			\definecolor{colorbrewer6}{RGB}{227,26,28}
			\definecolor{colorbrewer7}{RGB}{253,191,111}
			\definecolor{colorbrewer8}{RGB}{255,127,0}
			\definecolor{colorbrewer9}{RGB}{202,178,214}
		},
		colorbrewer values/10/.code={
			\definecolor{colorbrewer1}{RGB}{166,206,227}
			\definecolor{colorbrewer2}{RGB}{31,120,180}
			\definecolor{colorbrewer3}{RGB}{178,223,138}
			\definecolor{colorbrewer4}{RGB}{51,160,44}
			\definecolor{colorbrewer5}{RGB}{251,154,153}
			\definecolor{colorbrewer6}{RGB}{227,26,28}
			\definecolor{colorbrewer7}{RGB}{253,191,111}
			\definecolor{colorbrewer8}{RGB}{255,127,0}
			\definecolor{colorbrewer9}{RGB}{202,178,214}
			\definecolor{colorbrewer10}{RGB}{106,61,154}
		},
		colorbrewer values/11/.code={
			\definecolor{colorbrewer1}{RGB}{166,206,227}
			\definecolor{colorbrewer2}{RGB}{31,120,180}
			\definecolor{colorbrewer3}{RGB}{178,223,138}
			\definecolor{colorbrewer4}{RGB}{51,160,44}
			\definecolor{colorbrewer5}{RGB}{251,154,153}
			\definecolor{colorbrewer6}{RGB}{227,26,28}
			\definecolor{colorbrewer7}{RGB}{253,191,111}
			\definecolor{colorbrewer8}{RGB}{255,127,0}
			\definecolor{colorbrewer9}{RGB}{202,178,214}
			\definecolor{colorbrewer10}{RGB}{106,61,154}
			\definecolor{colorbrewer11}{RGB}{255,255,153}
		},
		colorbrewer values/12/.code={
			\definecolor{colorbrewer1}{RGB}{166,206,227}
			\definecolor{colorbrewer2}{RGB}{31,120,180}
			\definecolor{colorbrewer3}{RGB}{178,223,138}
			\definecolor{colorbrewer4}{RGB}{51,160,44}
			\definecolor{colorbrewer5}{RGB}{251,154,153}
			\definecolor{colorbrewer6}{RGB}{227,26,28}
			\definecolor{colorbrewer7}{RGB}{253,191,111}
			\definecolor{colorbrewer8}{RGB}{255,127,0}
			\definecolor{colorbrewer9}{RGB}{202,178,214}
			\definecolor{colorbrewer10}{RGB}{106,61,154}
			\definecolor{colorbrewer11}{RGB}{255,255,153}
			\definecolor{colorbrewer12}{RGB}{177,89,40}
		}
	},
	colorbrewer scheme/Pastel1/.style={
		colorbrewer values/.is choice,	
		colorbrewer values/3/.code={
			\definecolor{colorbrewer1}{RGB}{251,180,174}
			\definecolor{colorbrewer2}{RGB}{179,205,227}
			\definecolor{colorbrewer3}{RGB}{204,235,197}
		},
		colorbrewer values=3,
		colorbrewer values/4/.code={
			\definecolor{colorbrewer1}{RGB}{251,180,174}
			\definecolor{colorbrewer2}{RGB}{179,205,227}
			\definecolor{colorbrewer3}{RGB}{204,235,197}
			\definecolor{colorbrewer4}{RGB}{222,203,228}
		},
		colorbrewer values/5/.code={
			\definecolor{colorbrewer1}{RGB}{251,180,174}
			\definecolor{colorbrewer2}{RGB}{179,205,227}
			\definecolor{colorbrewer3}{RGB}{204,235,197}
			\definecolor{colorbrewer4}{RGB}{222,203,228}
			\definecolor{colorbrewer5}{RGB}{254,217,166}
		},
		colorbrewer values/6/.code={
			\definecolor{colorbrewer1}{RGB}{251,180,174}
			\definecolor{colorbrewer2}{RGB}{179,205,227}
			\definecolor{colorbrewer3}{RGB}{204,235,197}
			\definecolor{colorbrewer4}{RGB}{222,203,228}
			\definecolor{colorbrewer5}{RGB}{254,217,166}
			\definecolor{colorbrewer6}{RGB}{255,255,204}
		},
		colorbrewer values/7/.code={
			\definecolor{colorbrewer1}{RGB}{251,180,174}
			\definecolor{colorbrewer2}{RGB}{179,205,227}
			\definecolor{colorbrewer3}{RGB}{204,235,197}
			\definecolor{colorbrewer4}{RGB}{222,203,228}
			\definecolor{colorbrewer5}{RGB}{254,217,166}
			\definecolor{colorbrewer6}{RGB}{255,255,204}
			\definecolor{colorbrewer7}{RGB}{229,216,189}
		},
		colorbrewer values/8/.code={
			\definecolor{colorbrewer1}{RGB}{251,180,174}
			\definecolor{colorbrewer2}{RGB}{179,205,227}
			\definecolor{colorbrewer3}{RGB}{204,235,197}
			\definecolor{colorbrewer4}{RGB}{222,203,228}
			\definecolor{colorbrewer5}{RGB}{254,217,166}
			\definecolor{colorbrewer6}{RGB}{255,255,204}
			\definecolor{colorbrewer7}{RGB}{229,216,189}
			\definecolor{colorbrewer8}{RGB}{253,218,236}
		},
		colorbrewer values/9/.code={
			\definecolor{colorbrewer1}{RGB}{251,180,174}
			\definecolor{colorbrewer2}{RGB}{179,205,227}
			\definecolor{colorbrewer3}{RGB}{204,235,197}
			\definecolor{colorbrewer4}{RGB}{222,203,228}
			\definecolor{colorbrewer5}{RGB}{254,217,166}
			\definecolor{colorbrewer6}{RGB}{255,255,204}
			\definecolor{colorbrewer7}{RGB}{229,216,189}
			\definecolor{colorbrewer8}{RGB}{253,218,236}
			\definecolor{colorbrewer9}{RGB}{242,242,242}
		}
	},
	colorbrewer scheme/Pastel2/.style={
		colorbrewer values/.is choice,	
		colorbrewer values/3/.code={
			\definecolor{colorbrewer1}{RGB}{179,226,205}
			\definecolor{colorbrewer2}{RGB}{253,205,172}
			\definecolor{colorbrewer3}{RGB}{203,213,232}
		},
		colorbrewer values=3,
		colorbrewer values/4/.code={
			\definecolor{colorbrewer1}{RGB}{179,226,205}
			\definecolor{colorbrewer2}{RGB}{253,205,172}
			\definecolor{colorbrewer3}{RGB}{203,213,232}
			\definecolor{colorbrewer4}{RGB}{244,202,228}
		},
		colorbrewer values/5/.code={
			\definecolor{colorbrewer1}{RGB}{179,226,205}
			\definecolor{colorbrewer2}{RGB}{253,205,172}
			\definecolor{colorbrewer3}{RGB}{203,213,232}
			\definecolor{colorbrewer4}{RGB}{244,202,228}
			\definecolor{colorbrewer5}{RGB}{230,245,201}
		},
		colorbrewer values/6/.code={
			\definecolor{colorbrewer1}{RGB}{179,226,205}
			\definecolor{colorbrewer2}{RGB}{253,205,172}
			\definecolor{colorbrewer3}{RGB}{203,213,232}
			\definecolor{colorbrewer4}{RGB}{244,202,228}
			\definecolor{colorbrewer5}{RGB}{230,245,201}
			\definecolor{colorbrewer6}{RGB}{255,242,174}
		},
		colorbrewer values/7/.code={
			\definecolor{colorbrewer1}{RGB}{179,226,205}
			\definecolor{colorbrewer2}{RGB}{253,205,172}
			\definecolor{colorbrewer3}{RGB}{203,213,232}
			\definecolor{colorbrewer4}{RGB}{244,202,228}
			\definecolor{colorbrewer5}{RGB}{230,245,201}
			\definecolor{colorbrewer6}{RGB}{255,242,174}
			\definecolor{colorbrewer7}{RGB}{241,226,204}
		},
		colorbrewer values/8/.code={
			\definecolor{colorbrewer1}{RGB}{179,226,205}
			\definecolor{colorbrewer2}{RGB}{253,205,172}
			\definecolor{colorbrewer3}{RGB}{203,213,232}
			\definecolor{colorbrewer4}{RGB}{244,202,228}
			\definecolor{colorbrewer5}{RGB}{230,245,201}
			\definecolor{colorbrewer6}{RGB}{255,242,174}
			\definecolor{colorbrewer7}{RGB}{241,226,204}
			\definecolor{colorbrewer8}{RGB}{204,204,204}
		}
	},
	colorbrewer scheme/PiYG/.style={
		colorbrewer values/.is choice,	
		colorbrewer values/3/.code={
			\definecolor{colorbrewer1}{RGB}{233,163,201}
			\definecolor{colorbrewer2}{RGB}{247,247,247}
			\definecolor{colorbrewer3}{RGB}{161,215,106}
		},
		colorbrewer values=3,
		colorbrewer values/4/.code={
			\definecolor{colorbrewer1}{RGB}{208,28,139}
			\definecolor{colorbrewer2}{RGB}{241,182,218}
			\definecolor{colorbrewer3}{RGB}{184,225,134}
			\definecolor{colorbrewer4}{RGB}{77,172,38}
		},
		colorbrewer values/5/.code={
			\definecolor{colorbrewer1}{RGB}{208,28,139}
			\definecolor{colorbrewer2}{RGB}{241,182,218}
			\definecolor{colorbrewer3}{RGB}{247,247,247}
			\definecolor{colorbrewer4}{RGB}{184,225,134}
			\definecolor{colorbrewer5}{RGB}{77,172,38}
		},
		colorbrewer values/6/.code={
			\definecolor{colorbrewer1}{RGB}{197,27,125}
			\definecolor{colorbrewer2}{RGB}{233,163,201}
			\definecolor{colorbrewer3}{RGB}{253,224,239}
			\definecolor{colorbrewer4}{RGB}{230,245,208}
			\definecolor{colorbrewer5}{RGB}{161,215,106}
			\definecolor{colorbrewer6}{RGB}{77,146,33}
		},
		colorbrewer values/7/.code={
			\definecolor{colorbrewer1}{RGB}{197,27,125}
			\definecolor{colorbrewer2}{RGB}{233,163,201}
			\definecolor{colorbrewer3}{RGB}{253,224,239}
			\definecolor{colorbrewer4}{RGB}{247,247,247}
			\definecolor{colorbrewer5}{RGB}{230,245,208}
			\definecolor{colorbrewer6}{RGB}{161,215,106}
			\definecolor{colorbrewer7}{RGB}{77,146,33}
		},
		colorbrewer values/8/.code={
			\definecolor{colorbrewer1}{RGB}{197,27,125}
			\definecolor{colorbrewer2}{RGB}{222,119,174}
			\definecolor{colorbrewer3}{RGB}{241,182,218}
			\definecolor{colorbrewer4}{RGB}{253,224,239}
			\definecolor{colorbrewer5}{RGB}{230,245,208}
			\definecolor{colorbrewer6}{RGB}{184,225,134}
			\definecolor{colorbrewer7}{RGB}{127,188,65}
			\definecolor{colorbrewer8}{RGB}{77,146,33}
		},
		colorbrewer values/9/.code={
			\definecolor{colorbrewer1}{RGB}{197,27,125}
			\definecolor{colorbrewer2}{RGB}{222,119,174}
			\definecolor{colorbrewer3}{RGB}{241,182,218}
			\definecolor{colorbrewer4}{RGB}{253,224,239}
			\definecolor{colorbrewer5}{RGB}{247,247,247}
			\definecolor{colorbrewer6}{RGB}{230,245,208}
			\definecolor{colorbrewer7}{RGB}{184,225,134}
			\definecolor{colorbrewer8}{RGB}{127,188,65}
			\definecolor{colorbrewer9}{RGB}{77,146,33}
		},
		colorbrewer values/10/.code={
			\definecolor{colorbrewer1}{RGB}{142,1,82}
			\definecolor{colorbrewer2}{RGB}{197,27,125}
			\definecolor{colorbrewer3}{RGB}{222,119,174}
			\definecolor{colorbrewer4}{RGB}{241,182,218}
			\definecolor{colorbrewer5}{RGB}{253,224,239}
			\definecolor{colorbrewer6}{RGB}{230,245,208}
			\definecolor{colorbrewer7}{RGB}{184,225,134}
			\definecolor{colorbrewer8}{RGB}{127,188,65}
			\definecolor{colorbrewer9}{RGB}{77,146,33}
			\definecolor{colorbrewer10}{RGB}{39,100,25}
		},
		colorbrewer values/11/.code={
			\definecolor{colorbrewer1}{RGB}{142,1,82}
			\definecolor{colorbrewer2}{RGB}{197,27,125}
			\definecolor{colorbrewer3}{RGB}{222,119,174}
			\definecolor{colorbrewer4}{RGB}{241,182,218}
			\definecolor{colorbrewer5}{RGB}{253,224,239}
			\definecolor{colorbrewer6}{RGB}{247,247,247}
			\definecolor{colorbrewer7}{RGB}{230,245,208}
			\definecolor{colorbrewer8}{RGB}{184,225,134}
			\definecolor{colorbrewer9}{RGB}{127,188,65}
			\definecolor{colorbrewer10}{RGB}{77,146,33}
			\definecolor{colorbrewer11}{RGB}{39,100,25}
		}
	},
	colorbrewer scheme/PRGn/.style={
		colorbrewer values/.is choice,	
		colorbrewer values/3/.code={
			\definecolor{colorbrewer1}{RGB}{175,141,195}
			\definecolor{colorbrewer2}{RGB}{247,247,247}
			\definecolor{colorbrewer3}{RGB}{127,191,123}
		},
		colorbrewer values=3,
		colorbrewer values/4/.code={
			\definecolor{colorbrewer1}{RGB}{123,50,148}
			\definecolor{colorbrewer2}{RGB}{194,165,207}
			\definecolor{colorbrewer3}{RGB}{166,219,160}
			\definecolor{colorbrewer4}{RGB}{0,136,55}
		},
		colorbrewer values/5/.code={
			\definecolor{colorbrewer1}{RGB}{123,50,148}
			\definecolor{colorbrewer2}{RGB}{194,165,207}
			\definecolor{colorbrewer3}{RGB}{247,247,247}
			\definecolor{colorbrewer4}{RGB}{166,219,160}
			\definecolor{colorbrewer5}{RGB}{0,136,55}
		},
		colorbrewer values/6/.code={
			\definecolor{colorbrewer1}{RGB}{118,42,131}
			\definecolor{colorbrewer2}{RGB}{175,141,195}
			\definecolor{colorbrewer3}{RGB}{231,212,232}
			\definecolor{colorbrewer4}{RGB}{217,240,211}
			\definecolor{colorbrewer5}{RGB}{127,191,123}
			\definecolor{colorbrewer6}{RGB}{27,120,55}
		},
		colorbrewer values/7/.code={
			\definecolor{colorbrewer1}{RGB}{118,42,131}
			\definecolor{colorbrewer2}{RGB}{175,141,195}
			\definecolor{colorbrewer3}{RGB}{231,212,232}
			\definecolor{colorbrewer4}{RGB}{247,247,247}
			\definecolor{colorbrewer5}{RGB}{217,240,211}
			\definecolor{colorbrewer6}{RGB}{127,191,123}
			\definecolor{colorbrewer7}{RGB}{27,120,55}
		},
		colorbrewer values/8/.code={
			\definecolor{colorbrewer1}{RGB}{118,42,131}
			\definecolor{colorbrewer2}{RGB}{153,112,171}
			\definecolor{colorbrewer3}{RGB}{194,165,207}
			\definecolor{colorbrewer4}{RGB}{231,212,232}
			\definecolor{colorbrewer5}{RGB}{217,240,211}
			\definecolor{colorbrewer6}{RGB}{166,219,160}
			\definecolor{colorbrewer7}{RGB}{90,174,97}
			\definecolor{colorbrewer8}{RGB}{27,120,55}
		},
		colorbrewer values/9/.code={
			\definecolor{colorbrewer1}{RGB}{118,42,131}
			\definecolor{colorbrewer2}{RGB}{153,112,171}
			\definecolor{colorbrewer3}{RGB}{194,165,207}
			\definecolor{colorbrewer4}{RGB}{231,212,232}
			\definecolor{colorbrewer5}{RGB}{247,247,247}
			\definecolor{colorbrewer6}{RGB}{217,240,211}
			\definecolor{colorbrewer7}{RGB}{166,219,160}
			\definecolor{colorbrewer8}{RGB}{90,174,97}
			\definecolor{colorbrewer9}{RGB}{27,120,55}
		},
		colorbrewer values/10/.code={
			\definecolor{colorbrewer1}{RGB}{64,0,75}
			\definecolor{colorbrewer2}{RGB}{118,42,131}
			\definecolor{colorbrewer3}{RGB}{153,112,171}
			\definecolor{colorbrewer4}{RGB}{194,165,207}
			\definecolor{colorbrewer5}{RGB}{231,212,232}
			\definecolor{colorbrewer6}{RGB}{217,240,211}
			\definecolor{colorbrewer7}{RGB}{166,219,160}
			\definecolor{colorbrewer8}{RGB}{90,174,97}
			\definecolor{colorbrewer9}{RGB}{27,120,55}
			\definecolor{colorbrewer10}{RGB}{0,68,27}
		},
		colorbrewer values/11/.code={
			\definecolor{colorbrewer1}{RGB}{64,0,75}
			\definecolor{colorbrewer2}{RGB}{118,42,131}
			\definecolor{colorbrewer3}{RGB}{153,112,171}
			\definecolor{colorbrewer4}{RGB}{194,165,207}
			\definecolor{colorbrewer5}{RGB}{231,212,232}
			\definecolor{colorbrewer6}{RGB}{247,247,247}
			\definecolor{colorbrewer7}{RGB}{217,240,211}
			\definecolor{colorbrewer8}{RGB}{166,219,160}
			\definecolor{colorbrewer9}{RGB}{90,174,97}
			\definecolor{colorbrewer10}{RGB}{27,120,55}
			\definecolor{colorbrewer11}{RGB}{0,68,27}
		}
	},
	colorbrewer scheme/PuBu/.style={
		colorbrewer values/.is choice,	
		colorbrewer values/3/.code={
			\definecolor{colorbrewer1}{RGB}{236,231,242}
			\definecolor{colorbrewer2}{RGB}{166,189,219}
			\definecolor{colorbrewer3}{RGB}{43,140,190}
		},
		colorbrewer values=3,
		colorbrewer values/4/.code={
			\definecolor{colorbrewer1}{RGB}{241,238,246}
			\definecolor{colorbrewer2}{RGB}{189,201,225}
			\definecolor{colorbrewer3}{RGB}{116,169,207}
			\definecolor{colorbrewer4}{RGB}{5,112,176}
		},
		colorbrewer values/5/.code={
			\definecolor{colorbrewer1}{RGB}{241,238,246}
			\definecolor{colorbrewer2}{RGB}{189,201,225}
			\definecolor{colorbrewer3}{RGB}{116,169,207}
			\definecolor{colorbrewer4}{RGB}{43,140,190}
			\definecolor{colorbrewer5}{RGB}{4,90,141}
		},
		colorbrewer values/6/.code={
			\definecolor{colorbrewer1}{RGB}{241,238,246}
			\definecolor{colorbrewer2}{RGB}{208,209,230}
			\definecolor{colorbrewer3}{RGB}{166,189,219}
			\definecolor{colorbrewer4}{RGB}{116,169,207}
			\definecolor{colorbrewer5}{RGB}{43,140,190}
			\definecolor{colorbrewer6}{RGB}{4,90,141}
		},
		colorbrewer values/7/.code={
			\definecolor{colorbrewer1}{RGB}{241,238,246}
			\definecolor{colorbrewer2}{RGB}{208,209,230}
			\definecolor{colorbrewer3}{RGB}{166,189,219}
			\definecolor{colorbrewer4}{RGB}{116,169,207}
			\definecolor{colorbrewer5}{RGB}{54,144,192}
			\definecolor{colorbrewer6}{RGB}{5,112,176}
			\definecolor{colorbrewer7}{RGB}{3,78,123}
		},
		colorbrewer values/8/.code={
			\definecolor{colorbrewer1}{RGB}{255,247,251}
			\definecolor{colorbrewer2}{RGB}{236,231,242}
			\definecolor{colorbrewer3}{RGB}{208,209,230}
			\definecolor{colorbrewer4}{RGB}{166,189,219}
			\definecolor{colorbrewer5}{RGB}{116,169,207}
			\definecolor{colorbrewer6}{RGB}{54,144,192}
			\definecolor{colorbrewer7}{RGB}{5,112,176}
			\definecolor{colorbrewer8}{RGB}{3,78,123}
		},
		colorbrewer values/9/.code={
			\definecolor{colorbrewer1}{RGB}{255,247,251}
			\definecolor{colorbrewer2}{RGB}{236,231,242}
			\definecolor{colorbrewer3}{RGB}{208,209,230}
			\definecolor{colorbrewer4}{RGB}{166,189,219}
			\definecolor{colorbrewer5}{RGB}{116,169,207}
			\definecolor{colorbrewer6}{RGB}{54,144,192}
			\definecolor{colorbrewer7}{RGB}{5,112,176}
			\definecolor{colorbrewer8}{RGB}{4,90,141}
			\definecolor{colorbrewer9}{RGB}{2,56,88}
		}
	},
	colorbrewer scheme/PuBuGn/.style={
		colorbrewer values/.is choice,	
		colorbrewer values/3/.code={
			\definecolor{colorbrewer1}{RGB}{236,226,240}
			\definecolor{colorbrewer2}{RGB}{166,189,219}
			\definecolor{colorbrewer3}{RGB}{28,144,153}
		},
		colorbrewer values=3,
		colorbrewer values/4/.code={
			\definecolor{colorbrewer1}{RGB}{246,239,247}
			\definecolor{colorbrewer2}{RGB}{189,201,225}
			\definecolor{colorbrewer3}{RGB}{103,169,207}
			\definecolor{colorbrewer4}{RGB}{2,129,138}
		},
		colorbrewer values/5/.code={
			\definecolor{colorbrewer1}{RGB}{246,239,247}
			\definecolor{colorbrewer2}{RGB}{189,201,225}
			\definecolor{colorbrewer3}{RGB}{103,169,207}
			\definecolor{colorbrewer4}{RGB}{28,144,153}
			\definecolor{colorbrewer5}{RGB}{1,108,89}
		},
		colorbrewer values/6/.code={
			\definecolor{colorbrewer1}{RGB}{246,239,247}
			\definecolor{colorbrewer2}{RGB}{208,209,230}
			\definecolor{colorbrewer3}{RGB}{166,189,219}
			\definecolor{colorbrewer4}{RGB}{103,169,207}
			\definecolor{colorbrewer5}{RGB}{28,144,153}
			\definecolor{colorbrewer6}{RGB}{1,108,89}
		},
		colorbrewer values/7/.code={
			\definecolor{colorbrewer1}{RGB}{246,239,247}
			\definecolor{colorbrewer2}{RGB}{208,209,230}
			\definecolor{colorbrewer3}{RGB}{166,189,219}
			\definecolor{colorbrewer4}{RGB}{103,169,207}
			\definecolor{colorbrewer5}{RGB}{54,144,192}
			\definecolor{colorbrewer6}{RGB}{2,129,138}
			\definecolor{colorbrewer7}{RGB}{1,100,80}
		},
		colorbrewer values/8/.code={
			\definecolor{colorbrewer1}{RGB}{255,247,251}
			\definecolor{colorbrewer2}{RGB}{236,226,240}
			\definecolor{colorbrewer3}{RGB}{208,209,230}
			\definecolor{colorbrewer4}{RGB}{166,189,219}
			\definecolor{colorbrewer5}{RGB}{103,169,207}
			\definecolor{colorbrewer6}{RGB}{54,144,192}
			\definecolor{colorbrewer7}{RGB}{2,129,138}
			\definecolor{colorbrewer8}{RGB}{1,100,80}
		},
		colorbrewer values/9/.code={
			\definecolor{colorbrewer1}{RGB}{255,247,251}
			\definecolor{colorbrewer2}{RGB}{236,226,240}
			\definecolor{colorbrewer3}{RGB}{208,209,230}
			\definecolor{colorbrewer4}{RGB}{166,189,219}
			\definecolor{colorbrewer5}{RGB}{103,169,207}
			\definecolor{colorbrewer6}{RGB}{54,144,192}
			\definecolor{colorbrewer7}{RGB}{2,129,138}
			\definecolor{colorbrewer8}{RGB}{1,108,89}
			\definecolor{colorbrewer9}{RGB}{1,70,54}
		}
	},
	colorbrewer scheme/PuOr/.style={
		colorbrewer values/.is choice,	
		colorbrewer values/3/.code={
			\definecolor{colorbrewer1}{RGB}{241,163,64}
			\definecolor{colorbrewer2}{RGB}{247,247,247}
			\definecolor{colorbrewer3}{RGB}{153,142,195}
		},
		colorbrewer values=3,
		colorbrewer values/4/.code={
			\definecolor{colorbrewer1}{RGB}{230,97,1}
			\definecolor{colorbrewer2}{RGB}{253,184,99}
			\definecolor{colorbrewer3}{RGB}{178,171,210}
			\definecolor{colorbrewer4}{RGB}{94,60,153}
		},
		colorbrewer values/5/.code={
			\definecolor{colorbrewer1}{RGB}{230,97,1}
			\definecolor{colorbrewer2}{RGB}{253,184,99}
			\definecolor{colorbrewer3}{RGB}{247,247,247}
			\definecolor{colorbrewer4}{RGB}{178,171,210}
			\definecolor{colorbrewer5}{RGB}{94,60,153}
		},
		colorbrewer values/6/.code={
			\definecolor{colorbrewer1}{RGB}{179,88,6}
			\definecolor{colorbrewer2}{RGB}{241,163,64}
			\definecolor{colorbrewer3}{RGB}{254,224,182}
			\definecolor{colorbrewer4}{RGB}{216,218,235}
			\definecolor{colorbrewer5}{RGB}{153,142,195}
			\definecolor{colorbrewer6}{RGB}{84,39,136}
		},
		colorbrewer values/7/.code={
			\definecolor{colorbrewer1}{RGB}{179,88,6}
			\definecolor{colorbrewer2}{RGB}{241,163,64}
			\definecolor{colorbrewer3}{RGB}{254,224,182}
			\definecolor{colorbrewer4}{RGB}{247,247,247}
			\definecolor{colorbrewer5}{RGB}{216,218,235}
			\definecolor{colorbrewer6}{RGB}{153,142,195}
			\definecolor{colorbrewer7}{RGB}{84,39,136}
		},
		colorbrewer values/8/.code={
			\definecolor{colorbrewer1}{RGB}{179,88,6}
			\definecolor{colorbrewer2}{RGB}{224,130,20}
			\definecolor{colorbrewer3}{RGB}{253,184,99}
			\definecolor{colorbrewer4}{RGB}{254,224,182}
			\definecolor{colorbrewer5}{RGB}{216,218,235}
			\definecolor{colorbrewer6}{RGB}{178,171,210}
			\definecolor{colorbrewer7}{RGB}{128,115,172}
			\definecolor{colorbrewer8}{RGB}{84,39,136}
		},
		colorbrewer values/9/.code={
			\definecolor{colorbrewer1}{RGB}{179,88,6}
			\definecolor{colorbrewer2}{RGB}{224,130,20}
			\definecolor{colorbrewer3}{RGB}{253,184,99}
			\definecolor{colorbrewer4}{RGB}{254,224,182}
			\definecolor{colorbrewer5}{RGB}{247,247,247}
			\definecolor{colorbrewer6}{RGB}{216,218,235}
			\definecolor{colorbrewer7}{RGB}{178,171,210}
			\definecolor{colorbrewer8}{RGB}{128,115,172}
			\definecolor{colorbrewer9}{RGB}{84,39,136}
		},
		colorbrewer values/10/.code={
			\definecolor{colorbrewer1}{RGB}{127,59,8}
			\definecolor{colorbrewer2}{RGB}{179,88,6}
			\definecolor{colorbrewer3}{RGB}{224,130,20}
			\definecolor{colorbrewer4}{RGB}{253,184,99}
			\definecolor{colorbrewer5}{RGB}{254,224,182}
			\definecolor{colorbrewer6}{RGB}{216,218,235}
			\definecolor{colorbrewer7}{RGB}{178,171,210}
			\definecolor{colorbrewer8}{RGB}{128,115,172}
			\definecolor{colorbrewer9}{RGB}{84,39,136}
			\definecolor{colorbrewer10}{RGB}{45,0,75}
		},
		colorbrewer values/11/.code={
			\definecolor{colorbrewer1}{RGB}{127,59,8}
			\definecolor{colorbrewer2}{RGB}{179,88,6}
			\definecolor{colorbrewer3}{RGB}{224,130,20}
			\definecolor{colorbrewer4}{RGB}{253,184,99}
			\definecolor{colorbrewer5}{RGB}{254,224,182}
			\definecolor{colorbrewer6}{RGB}{247,247,247}
			\definecolor{colorbrewer7}{RGB}{216,218,235}
			\definecolor{colorbrewer8}{RGB}{178,171,210}
			\definecolor{colorbrewer9}{RGB}{128,115,172}
			\definecolor{colorbrewer10}{RGB}{84,39,136}
			\definecolor{colorbrewer11}{RGB}{45,0,75}
		}
	},
	colorbrewer scheme/PuRd/.style={
		colorbrewer values/.is choice,	
		colorbrewer values/3/.code={
			\definecolor{colorbrewer1}{RGB}{231,225,239}
			\definecolor{colorbrewer2}{RGB}{201,148,199}
			\definecolor{colorbrewer3}{RGB}{221,28,119}
		},
		colorbrewer values=3,
		colorbrewer values/4/.code={
			\definecolor{colorbrewer1}{RGB}{241,238,246}
			\definecolor{colorbrewer2}{RGB}{215,181,216}
			\definecolor{colorbrewer3}{RGB}{223,101,176}
			\definecolor{colorbrewer4}{RGB}{206,18,86}
		},
		colorbrewer values/5/.code={
			\definecolor{colorbrewer1}{RGB}{241,238,246}
			\definecolor{colorbrewer2}{RGB}{215,181,216}
			\definecolor{colorbrewer3}{RGB}{223,101,176}
			\definecolor{colorbrewer4}{RGB}{221,28,119}
			\definecolor{colorbrewer5}{RGB}{152,0,67}
		},
		colorbrewer values/6/.code={
			\definecolor{colorbrewer1}{RGB}{241,238,246}
			\definecolor{colorbrewer2}{RGB}{212,185,218}
			\definecolor{colorbrewer3}{RGB}{201,148,199}
			\definecolor{colorbrewer4}{RGB}{223,101,176}
			\definecolor{colorbrewer5}{RGB}{221,28,119}
			\definecolor{colorbrewer6}{RGB}{152,0,67}
		},
		colorbrewer values/7/.code={
			\definecolor{colorbrewer1}{RGB}{241,238,246}
			\definecolor{colorbrewer2}{RGB}{212,185,218}
			\definecolor{colorbrewer3}{RGB}{201,148,199}
			\definecolor{colorbrewer4}{RGB}{223,101,176}
			\definecolor{colorbrewer5}{RGB}{231,41,138}
			\definecolor{colorbrewer6}{RGB}{206,18,86}
			\definecolor{colorbrewer7}{RGB}{145,0,63}
		},
		colorbrewer values/8/.code={
			\definecolor{colorbrewer1}{RGB}{247,244,249}
			\definecolor{colorbrewer2}{RGB}{231,225,239}
			\definecolor{colorbrewer3}{RGB}{212,185,218}
			\definecolor{colorbrewer4}{RGB}{201,148,199}
			\definecolor{colorbrewer5}{RGB}{223,101,176}
			\definecolor{colorbrewer6}{RGB}{231,41,138}
			\definecolor{colorbrewer7}{RGB}{206,18,86}
			\definecolor{colorbrewer8}{RGB}{145,0,63}
		},
		colorbrewer values/9/.code={
			\definecolor{colorbrewer1}{RGB}{247,244,249}
			\definecolor{colorbrewer2}{RGB}{231,225,239}
			\definecolor{colorbrewer3}{RGB}{212,185,218}
			\definecolor{colorbrewer4}{RGB}{201,148,199}
			\definecolor{colorbrewer5}{RGB}{223,101,176}
			\definecolor{colorbrewer6}{RGB}{231,41,138}
			\definecolor{colorbrewer7}{RGB}{206,18,86}
			\definecolor{colorbrewer8}{RGB}{152,0,67}
			\definecolor{colorbrewer9}{RGB}{103,0,31}
		}
	},
	colorbrewer scheme/Purples/.style={
		colorbrewer values/.is choice,	
		colorbrewer values/3/.code={
			\definecolor{colorbrewer1}{RGB}{239,237,245}
			\definecolor{colorbrewer2}{RGB}{188,189,220}
			\definecolor{colorbrewer3}{RGB}{117,107,177}
		},
		colorbrewer values=3,
		colorbrewer values/4/.code={
			\definecolor{colorbrewer1}{RGB}{242,240,247}
			\definecolor{colorbrewer2}{RGB}{203,201,226}
			\definecolor{colorbrewer3}{RGB}{158,154,200}
			\definecolor{colorbrewer4}{RGB}{106,81,163}
		},
		colorbrewer values/5/.code={
			\definecolor{colorbrewer1}{RGB}{242,240,247}
			\definecolor{colorbrewer2}{RGB}{203,201,226}
			\definecolor{colorbrewer3}{RGB}{158,154,200}
			\definecolor{colorbrewer4}{RGB}{117,107,177}
			\definecolor{colorbrewer5}{RGB}{84,39,143}
		},
		colorbrewer values/6/.code={
			\definecolor{colorbrewer1}{RGB}{242,240,247}
			\definecolor{colorbrewer2}{RGB}{218,218,235}
			\definecolor{colorbrewer3}{RGB}{188,189,220}
			\definecolor{colorbrewer4}{RGB}{158,154,200}
			\definecolor{colorbrewer5}{RGB}{117,107,177}
			\definecolor{colorbrewer6}{RGB}{84,39,143}
		},
		colorbrewer values/7/.code={
			\definecolor{colorbrewer1}{RGB}{242,240,247}
			\definecolor{colorbrewer2}{RGB}{218,218,235}
			\definecolor{colorbrewer3}{RGB}{188,189,220}
			\definecolor{colorbrewer4}{RGB}{158,154,200}
			\definecolor{colorbrewer5}{RGB}{128,125,186}
			\definecolor{colorbrewer6}{RGB}{106,81,163}
			\definecolor{colorbrewer7}{RGB}{74,20,134}
		},
		colorbrewer values/8/.code={
			\definecolor{colorbrewer1}{RGB}{252,251,253}
			\definecolor{colorbrewer2}{RGB}{239,237,245}
			\definecolor{colorbrewer3}{RGB}{218,218,235}
			\definecolor{colorbrewer4}{RGB}{188,189,220}
			\definecolor{colorbrewer5}{RGB}{158,154,200}
			\definecolor{colorbrewer6}{RGB}{128,125,186}
			\definecolor{colorbrewer7}{RGB}{106,81,163}
			\definecolor{colorbrewer8}{RGB}{74,20,134}
		},
		colorbrewer values/9/.code={
			\definecolor{colorbrewer1}{RGB}{252,251,253}
			\definecolor{colorbrewer2}{RGB}{239,237,245}
			\definecolor{colorbrewer3}{RGB}{218,218,235}
			\definecolor{colorbrewer4}{RGB}{188,189,220}
			\definecolor{colorbrewer5}{RGB}{158,154,200}
			\definecolor{colorbrewer6}{RGB}{128,125,186}
			\definecolor{colorbrewer7}{RGB}{106,81,163}
			\definecolor{colorbrewer8}{RGB}{84,39,143}
			\definecolor{colorbrewer9}{RGB}{63,0,125}
		}
	},
	colorbrewer scheme/RdBu/.style={
		colorbrewer values/.is choice,	
		colorbrewer values/3/.code={
			\definecolor{colorbrewer1}{RGB}{239,138,98}
			\definecolor{colorbrewer2}{RGB}{247,247,247}
			\definecolor{colorbrewer3}{RGB}{103,169,207}
		},
		colorbrewer values=3,
		colorbrewer values/4/.code={
			\definecolor{colorbrewer1}{RGB}{202,0,32}
			\definecolor{colorbrewer2}{RGB}{244,165,130}
			\definecolor{colorbrewer3}{RGB}{146,197,222}
			\definecolor{colorbrewer4}{RGB}{5,113,176}
		},
		colorbrewer values/5/.code={
			\definecolor{colorbrewer1}{RGB}{202,0,32}
			\definecolor{colorbrewer2}{RGB}{244,165,130}
			\definecolor{colorbrewer3}{RGB}{247,247,247}
			\definecolor{colorbrewer4}{RGB}{146,197,222}
			\definecolor{colorbrewer5}{RGB}{5,113,176}
		},
		colorbrewer values/6/.code={
			\definecolor{colorbrewer1}{RGB}{178,24,43}
			\definecolor{colorbrewer2}{RGB}{239,138,98}
			\definecolor{colorbrewer3}{RGB}{253,219,199}
			\definecolor{colorbrewer4}{RGB}{209,229,240}
			\definecolor{colorbrewer5}{RGB}{103,169,207}
			\definecolor{colorbrewer6}{RGB}{33,102,172}
		},
		colorbrewer values/7/.code={
			\definecolor{colorbrewer1}{RGB}{178,24,43}
			\definecolor{colorbrewer2}{RGB}{239,138,98}
			\definecolor{colorbrewer3}{RGB}{253,219,199}
			\definecolor{colorbrewer4}{RGB}{247,247,247}
			\definecolor{colorbrewer5}{RGB}{209,229,240}
			\definecolor{colorbrewer6}{RGB}{103,169,207}
			\definecolor{colorbrewer7}{RGB}{33,102,172}
		},
		colorbrewer values/8/.code={
			\definecolor{colorbrewer1}{RGB}{178,24,43}
			\definecolor{colorbrewer2}{RGB}{214,96,77}
			\definecolor{colorbrewer3}{RGB}{244,165,130}
			\definecolor{colorbrewer4}{RGB}{253,219,199}
			\definecolor{colorbrewer5}{RGB}{209,229,240}
			\definecolor{colorbrewer6}{RGB}{146,197,222}
			\definecolor{colorbrewer7}{RGB}{67,147,195}
			\definecolor{colorbrewer8}{RGB}{33,102,172}
		},
		colorbrewer values/9/.code={
			\definecolor{colorbrewer1}{RGB}{178,24,43}
			\definecolor{colorbrewer2}{RGB}{214,96,77}
			\definecolor{colorbrewer3}{RGB}{244,165,130}
			\definecolor{colorbrewer4}{RGB}{253,219,199}
			\definecolor{colorbrewer5}{RGB}{247,247,247}
			\definecolor{colorbrewer6}{RGB}{209,229,240}
			\definecolor{colorbrewer7}{RGB}{146,197,222}
			\definecolor{colorbrewer8}{RGB}{67,147,195}
			\definecolor{colorbrewer9}{RGB}{33,102,172}
		},
		colorbrewer values/10/.code={
			\definecolor{colorbrewer1}{RGB}{103,0,31}
			\definecolor{colorbrewer2}{RGB}{178,24,43}
			\definecolor{colorbrewer3}{RGB}{214,96,77}
			\definecolor{colorbrewer4}{RGB}{244,165,130}
			\definecolor{colorbrewer5}{RGB}{253,219,199}
			\definecolor{colorbrewer6}{RGB}{209,229,240}
			\definecolor{colorbrewer7}{RGB}{146,197,222}
			\definecolor{colorbrewer8}{RGB}{67,147,195}
			\definecolor{colorbrewer9}{RGB}{33,102,172}
			\definecolor{colorbrewer10}{RGB}{5,48,97}
		},
		colorbrewer values/11/.code={
			\definecolor{colorbrewer1}{RGB}{103,0,31}
			\definecolor{colorbrewer2}{RGB}{178,24,43}
			\definecolor{colorbrewer3}{RGB}{214,96,77}
			\definecolor{colorbrewer4}{RGB}{244,165,130}
			\definecolor{colorbrewer5}{RGB}{253,219,199}
			\definecolor{colorbrewer6}{RGB}{247,247,247}
			\definecolor{colorbrewer7}{RGB}{209,229,240}
			\definecolor{colorbrewer8}{RGB}{146,197,222}
			\definecolor{colorbrewer9}{RGB}{67,147,195}
			\definecolor{colorbrewer10}{RGB}{33,102,172}
			\definecolor{colorbrewer11}{RGB}{5,48,97}
		}
	},
	colorbrewer scheme/RdGy/.style={
		colorbrewer values/.is choice,	
		colorbrewer values/3/.code={
			\definecolor{colorbrewer1}{RGB}{239,138,98}
			\definecolor{colorbrewer2}{RGB}{255,255,255}
			\definecolor{colorbrewer3}{RGB}{153,153,153}
		},
		colorbrewer values=3,
		colorbrewer values/4/.code={
			\definecolor{colorbrewer1}{RGB}{202,0,32}
			\definecolor{colorbrewer2}{RGB}{244,165,130}
			\definecolor{colorbrewer3}{RGB}{186,186,186}
			\definecolor{colorbrewer4}{RGB}{64,64,64}
		},
		colorbrewer values/5/.code={
			\definecolor{colorbrewer1}{RGB}{202,0,32}
			\definecolor{colorbrewer2}{RGB}{244,165,130}
			\definecolor{colorbrewer3}{RGB}{255,255,255}
			\definecolor{colorbrewer4}{RGB}{186,186,186}
			\definecolor{colorbrewer5}{RGB}{64,64,64}
		},
		colorbrewer values/6/.code={
			\definecolor{colorbrewer1}{RGB}{178,24,43}
			\definecolor{colorbrewer2}{RGB}{239,138,98}
			\definecolor{colorbrewer3}{RGB}{253,219,199}
			\definecolor{colorbrewer4}{RGB}{224,224,224}
			\definecolor{colorbrewer5}{RGB}{153,153,153}
			\definecolor{colorbrewer6}{RGB}{77,77,77}
		},
		colorbrewer values/7/.code={
			\definecolor{colorbrewer1}{RGB}{178,24,43}
			\definecolor{colorbrewer2}{RGB}{239,138,98}
			\definecolor{colorbrewer3}{RGB}{253,219,199}
			\definecolor{colorbrewer4}{RGB}{255,255,255}
			\definecolor{colorbrewer5}{RGB}{224,224,224}
			\definecolor{colorbrewer6}{RGB}{153,153,153}
			\definecolor{colorbrewer7}{RGB}{77,77,77}
		},
		colorbrewer values/8/.code={
			\definecolor{colorbrewer1}{RGB}{178,24,43}
			\definecolor{colorbrewer2}{RGB}{214,96,77}
			\definecolor{colorbrewer3}{RGB}{244,165,130}
			\definecolor{colorbrewer4}{RGB}{253,219,199}
			\definecolor{colorbrewer5}{RGB}{224,224,224}
			\definecolor{colorbrewer6}{RGB}{186,186,186}
			\definecolor{colorbrewer7}{RGB}{135,135,135}
			\definecolor{colorbrewer8}{RGB}{77,77,77}
		},
		colorbrewer values/9/.code={
			\definecolor{colorbrewer1}{RGB}{178,24,43}
			\definecolor{colorbrewer2}{RGB}{214,96,77}
			\definecolor{colorbrewer3}{RGB}{244,165,130}
			\definecolor{colorbrewer4}{RGB}{253,219,199}
			\definecolor{colorbrewer5}{RGB}{255,255,255}
			\definecolor{colorbrewer6}{RGB}{224,224,224}
			\definecolor{colorbrewer7}{RGB}{186,186,186}
			\definecolor{colorbrewer8}{RGB}{135,135,135}
			\definecolor{colorbrewer9}{RGB}{77,77,77}
		},
		colorbrewer values/10/.code={
			\definecolor{colorbrewer1}{RGB}{103,0,31}
			\definecolor{colorbrewer2}{RGB}{178,24,43}
			\definecolor{colorbrewer3}{RGB}{214,96,77}
			\definecolor{colorbrewer4}{RGB}{244,165,130}
			\definecolor{colorbrewer5}{RGB}{253,219,199}
			\definecolor{colorbrewer6}{RGB}{224,224,224}
			\definecolor{colorbrewer7}{RGB}{186,186,186}
			\definecolor{colorbrewer8}{RGB}{135,135,135}
			\definecolor{colorbrewer9}{RGB}{77,77,77}
			\definecolor{colorbrewer10}{RGB}{26,26,26}
		},
		colorbrewer values/11/.code={
			\definecolor{colorbrewer1}{RGB}{103,0,31}
			\definecolor{colorbrewer2}{RGB}{178,24,43}
			\definecolor{colorbrewer3}{RGB}{214,96,77}
			\definecolor{colorbrewer4}{RGB}{244,165,130}
			\definecolor{colorbrewer5}{RGB}{253,219,199}
			\definecolor{colorbrewer6}{RGB}{255,255,255}
			\definecolor{colorbrewer7}{RGB}{224,224,224}
			\definecolor{colorbrewer8}{RGB}{186,186,186}
			\definecolor{colorbrewer9}{RGB}{135,135,135}
			\definecolor{colorbrewer10}{RGB}{77,77,77}
			\definecolor{colorbrewer11}{RGB}{26,26,26}
		}
	},
	colorbrewer scheme/RdPu/.style={
		colorbrewer values/.is choice,	
		colorbrewer values/3/.code={
			\definecolor{colorbrewer1}{RGB}{253,224,221}
			\definecolor{colorbrewer2}{RGB}{250,159,181}
			\definecolor{colorbrewer3}{RGB}{197,27,138}
		},
		colorbrewer values=3,
		colorbrewer values/4/.code={
			\definecolor{colorbrewer1}{RGB}{254,235,226}
			\definecolor{colorbrewer2}{RGB}{251,180,185}
			\definecolor{colorbrewer3}{RGB}{247,104,161}
			\definecolor{colorbrewer4}{RGB}{174,1,126}
		},
		colorbrewer values/5/.code={
			\definecolor{colorbrewer1}{RGB}{254,235,226}
			\definecolor{colorbrewer2}{RGB}{251,180,185}
			\definecolor{colorbrewer3}{RGB}{247,104,161}
			\definecolor{colorbrewer4}{RGB}{197,27,138}
			\definecolor{colorbrewer5}{RGB}{122,1,119}
		},
		colorbrewer values/6/.code={
			\definecolor{colorbrewer1}{RGB}{254,235,226}
			\definecolor{colorbrewer2}{RGB}{252,197,192}
			\definecolor{colorbrewer3}{RGB}{250,159,181}
			\definecolor{colorbrewer4}{RGB}{247,104,161}
			\definecolor{colorbrewer5}{RGB}{197,27,138}
			\definecolor{colorbrewer6}{RGB}{122,1,119}
		},
		colorbrewer values/7/.code={
			\definecolor{colorbrewer1}{RGB}{254,235,226}
			\definecolor{colorbrewer2}{RGB}{252,197,192}
			\definecolor{colorbrewer3}{RGB}{250,159,181}
			\definecolor{colorbrewer4}{RGB}{247,104,161}
			\definecolor{colorbrewer5}{RGB}{221,52,151}
			\definecolor{colorbrewer6}{RGB}{174,1,126}
			\definecolor{colorbrewer7}{RGB}{122,1,119}
		},
		colorbrewer values/8/.code={
			\definecolor{colorbrewer1}{RGB}{255,247,243}
			\definecolor{colorbrewer2}{RGB}{253,224,221}
			\definecolor{colorbrewer3}{RGB}{252,197,192}
			\definecolor{colorbrewer4}{RGB}{250,159,181}
			\definecolor{colorbrewer5}{RGB}{247,104,161}
			\definecolor{colorbrewer6}{RGB}{221,52,151}
			\definecolor{colorbrewer7}{RGB}{174,1,126}
			\definecolor{colorbrewer8}{RGB}{122,1,119}
		},
		colorbrewer values/9/.code={
			\definecolor{colorbrewer1}{RGB}{255,247,243}
			\definecolor{colorbrewer2}{RGB}{253,224,221}
			\definecolor{colorbrewer3}{RGB}{252,197,192}
			\definecolor{colorbrewer4}{RGB}{250,159,181}
			\definecolor{colorbrewer5}{RGB}{247,104,161}
			\definecolor{colorbrewer6}{RGB}{221,52,151}
			\definecolor{colorbrewer7}{RGB}{174,1,126}
			\definecolor{colorbrewer8}{RGB}{122,1,119}
			\definecolor{colorbrewer9}{RGB}{73,0,106}
		}
	},
	colorbrewer scheme/Reds/.style={
		colorbrewer values/.is choice,	
		colorbrewer values/3/.code={
			\definecolor{colorbrewer1}{RGB}{254,224,210}
			\definecolor{colorbrewer2}{RGB}{252,146,114}
			\definecolor{colorbrewer3}{RGB}{222,45,38}
		},
		colorbrewer values=3,
		colorbrewer values/4/.code={
			\definecolor{colorbrewer1}{RGB}{254,229,217}
			\definecolor{colorbrewer2}{RGB}{252,174,145}
			\definecolor{colorbrewer3}{RGB}{251,106,74}
			\definecolor{colorbrewer4}{RGB}{203,24,29}
		},
		colorbrewer values/5/.code={
			\definecolor{colorbrewer1}{RGB}{254,229,217}
			\definecolor{colorbrewer2}{RGB}{252,174,145}
			\definecolor{colorbrewer3}{RGB}{251,106,74}
			\definecolor{colorbrewer4}{RGB}{222,45,38}
			\definecolor{colorbrewer5}{RGB}{165,15,21}
		},
		colorbrewer values/6/.code={
			\definecolor{colorbrewer1}{RGB}{254,229,217}
			\definecolor{colorbrewer2}{RGB}{252,187,161}
			\definecolor{colorbrewer3}{RGB}{252,146,114}
			\definecolor{colorbrewer4}{RGB}{251,106,74}
			\definecolor{colorbrewer5}{RGB}{222,45,38}
			\definecolor{colorbrewer6}{RGB}{165,15,21}
		},
		colorbrewer values/7/.code={
			\definecolor{colorbrewer1}{RGB}{254,229,217}
			\definecolor{colorbrewer2}{RGB}{252,187,161}
			\definecolor{colorbrewer3}{RGB}{252,146,114}
			\definecolor{colorbrewer4}{RGB}{251,106,74}
			\definecolor{colorbrewer5}{RGB}{239,59,44}
			\definecolor{colorbrewer6}{RGB}{203,24,29}
			\definecolor{colorbrewer7}{RGB}{153,0,13}
		},
		colorbrewer values/8/.code={
			\definecolor{colorbrewer1}{RGB}{255,245,240}
			\definecolor{colorbrewer2}{RGB}{254,224,210}
			\definecolor{colorbrewer3}{RGB}{252,187,161}
			\definecolor{colorbrewer4}{RGB}{252,146,114}
			\definecolor{colorbrewer5}{RGB}{251,106,74}
			\definecolor{colorbrewer6}{RGB}{239,59,44}
			\definecolor{colorbrewer7}{RGB}{203,24,29}
			\definecolor{colorbrewer8}{RGB}{153,0,13}
		},
		colorbrewer values/9/.code={
			\definecolor{colorbrewer1}{RGB}{255,245,240}
			\definecolor{colorbrewer2}{RGB}{254,224,210}
			\definecolor{colorbrewer3}{RGB}{252,187,161}
			\definecolor{colorbrewer4}{RGB}{252,146,114}
			\definecolor{colorbrewer5}{RGB}{251,106,74}
			\definecolor{colorbrewer6}{RGB}{239,59,44}
			\definecolor{colorbrewer7}{RGB}{203,24,29}
			\definecolor{colorbrewer8}{RGB}{165,15,21}
			\definecolor{colorbrewer9}{RGB}{103,0,13}
		}
	},
	colorbrewer scheme/RdYlBu/.style={
		colorbrewer values/.is choice,	
		colorbrewer values/3/.code={
			\definecolor{colorbrewer1}{RGB}{252,141,89}
			\definecolor{colorbrewer2}{RGB}{255,255,191}
			\definecolor{colorbrewer3}{RGB}{145,191,219}
		},
		colorbrewer values=3,
		colorbrewer values/4/.code={
			\definecolor{colorbrewer1}{RGB}{215,25,28}
			\definecolor{colorbrewer2}{RGB}{253,174,97}
			\definecolor{colorbrewer3}{RGB}{171,217,233}
			\definecolor{colorbrewer4}{RGB}{44,123,182}
		},
		colorbrewer values/5/.code={
			\definecolor{colorbrewer1}{RGB}{215,25,28}
			\definecolor{colorbrewer2}{RGB}{253,174,97}
			\definecolor{colorbrewer3}{RGB}{255,255,191}
			\definecolor{colorbrewer4}{RGB}{171,217,233}
			\definecolor{colorbrewer5}{RGB}{44,123,182}
		},
		colorbrewer values/6/.code={
			\definecolor{colorbrewer1}{RGB}{215,48,39}
			\definecolor{colorbrewer2}{RGB}{252,141,89}
			\definecolor{colorbrewer3}{RGB}{254,224,144}
			\definecolor{colorbrewer4}{RGB}{224,243,248}
			\definecolor{colorbrewer5}{RGB}{145,191,219}
			\definecolor{colorbrewer6}{RGB}{69,117,180}
		},
		colorbrewer values/7/.code={
			\definecolor{colorbrewer1}{RGB}{215,48,39}
			\definecolor{colorbrewer2}{RGB}{252,141,89}
			\definecolor{colorbrewer3}{RGB}{254,224,144}
			\definecolor{colorbrewer4}{RGB}{255,255,191}
			\definecolor{colorbrewer5}{RGB}{224,243,248}
			\definecolor{colorbrewer6}{RGB}{145,191,219}
			\definecolor{colorbrewer7}{RGB}{69,117,180}
		},
		colorbrewer values/8/.code={
			\definecolor{colorbrewer1}{RGB}{215,48,39}
			\definecolor{colorbrewer2}{RGB}{244,109,67}
			\definecolor{colorbrewer3}{RGB}{253,174,97}
			\definecolor{colorbrewer4}{RGB}{254,224,144}
			\definecolor{colorbrewer5}{RGB}{224,243,248}
			\definecolor{colorbrewer6}{RGB}{171,217,233}
			\definecolor{colorbrewer7}{RGB}{116,173,209}
			\definecolor{colorbrewer8}{RGB}{69,117,180}
		},
		colorbrewer values/9/.code={
			\definecolor{colorbrewer1}{RGB}{215,48,39}
			\definecolor{colorbrewer2}{RGB}{244,109,67}
			\definecolor{colorbrewer3}{RGB}{253,174,97}
			\definecolor{colorbrewer4}{RGB}{254,224,144}
			\definecolor{colorbrewer5}{RGB}{255,255,191}
			\definecolor{colorbrewer6}{RGB}{224,243,248}
			\definecolor{colorbrewer7}{RGB}{171,217,233}
			\definecolor{colorbrewer8}{RGB}{116,173,209}
			\definecolor{colorbrewer9}{RGB}{69,117,180}
		},
		colorbrewer values/10/.code={
			\definecolor{colorbrewer1}{RGB}{165,0,38}
			\definecolor{colorbrewer2}{RGB}{215,48,39}
			\definecolor{colorbrewer3}{RGB}{244,109,67}
			\definecolor{colorbrewer4}{RGB}{253,174,97}
			\definecolor{colorbrewer5}{RGB}{254,224,144}
			\definecolor{colorbrewer6}{RGB}{224,243,248}
			\definecolor{colorbrewer7}{RGB}{171,217,233}
			\definecolor{colorbrewer8}{RGB}{116,173,209}
			\definecolor{colorbrewer9}{RGB}{69,117,180}
			\definecolor{colorbrewer10}{RGB}{49,54,149}
		},
		colorbrewer values/11/.code={
			\definecolor{colorbrewer1}{RGB}{165,0,38}
			\definecolor{colorbrewer2}{RGB}{215,48,39}
			\definecolor{colorbrewer3}{RGB}{244,109,67}
			\definecolor{colorbrewer4}{RGB}{253,174,97}
			\definecolor{colorbrewer5}{RGB}{254,224,144}
			\definecolor{colorbrewer6}{RGB}{255,255,191}
			\definecolor{colorbrewer7}{RGB}{224,243,248}
			\definecolor{colorbrewer8}{RGB}{171,217,233}
			\definecolor{colorbrewer9}{RGB}{116,173,209}
			\definecolor{colorbrewer10}{RGB}{69,117,180}
			\definecolor{colorbrewer11}{RGB}{49,54,149}
		}
	},
	colorbrewer scheme/RdYlGn/.style={
		colorbrewer values/.is choice,	
		colorbrewer values/3/.code={
			\definecolor{colorbrewer1}{RGB}{252,141,89}
			\definecolor{colorbrewer2}{RGB}{255,255,191}
			\definecolor{colorbrewer3}{RGB}{145,207,96}
		},
		colorbrewer values=3,
		colorbrewer values/4/.code={
			\definecolor{colorbrewer1}{RGB}{215,25,28}
			\definecolor{colorbrewer2}{RGB}{253,174,97}
			\definecolor{colorbrewer3}{RGB}{166,217,106}
			\definecolor{colorbrewer4}{RGB}{26,150,65}
		},
		colorbrewer values/5/.code={
			\definecolor{colorbrewer1}{RGB}{215,25,28}
			\definecolor{colorbrewer2}{RGB}{253,174,97}
			\definecolor{colorbrewer3}{RGB}{255,255,191}
			\definecolor{colorbrewer4}{RGB}{166,217,106}
			\definecolor{colorbrewer5}{RGB}{26,150,65}
		},
		colorbrewer values/6/.code={
			\definecolor{colorbrewer1}{RGB}{215,48,39}
			\definecolor{colorbrewer2}{RGB}{252,141,89}
			\definecolor{colorbrewer3}{RGB}{254,224,139}
			\definecolor{colorbrewer4}{RGB}{217,239,139}
			\definecolor{colorbrewer5}{RGB}{145,207,96}
			\definecolor{colorbrewer6}{RGB}{26,152,80}
		},
		colorbrewer values/7/.code={
			\definecolor{colorbrewer1}{RGB}{215,48,39}
			\definecolor{colorbrewer2}{RGB}{252,141,89}
			\definecolor{colorbrewer3}{RGB}{254,224,139}
			\definecolor{colorbrewer4}{RGB}{255,255,191}
			\definecolor{colorbrewer5}{RGB}{217,239,139}
			\definecolor{colorbrewer6}{RGB}{145,207,96}
			\definecolor{colorbrewer7}{RGB}{26,152,80}
		},
		colorbrewer values/8/.code={
			\definecolor{colorbrewer1}{RGB}{215,48,39}
			\definecolor{colorbrewer2}{RGB}{244,109,67}
			\definecolor{colorbrewer3}{RGB}{253,174,97}
			\definecolor{colorbrewer4}{RGB}{254,224,139}
			\definecolor{colorbrewer5}{RGB}{217,239,139}
			\definecolor{colorbrewer6}{RGB}{166,217,106}
			\definecolor{colorbrewer7}{RGB}{102,189,99}
			\definecolor{colorbrewer8}{RGB}{26,152,80}
		},
		colorbrewer values/9/.code={
			\definecolor{colorbrewer1}{RGB}{215,48,39}
			\definecolor{colorbrewer2}{RGB}{244,109,67}
			\definecolor{colorbrewer3}{RGB}{253,174,97}
			\definecolor{colorbrewer4}{RGB}{254,224,139}
			\definecolor{colorbrewer5}{RGB}{255,255,191}
			\definecolor{colorbrewer6}{RGB}{217,239,139}
			\definecolor{colorbrewer7}{RGB}{166,217,106}
			\definecolor{colorbrewer8}{RGB}{102,189,99}
			\definecolor{colorbrewer9}{RGB}{26,152,80}
		},
		colorbrewer values/10/.code={
			\definecolor{colorbrewer1}{RGB}{165,0,38}
			\definecolor{colorbrewer2}{RGB}{215,48,39}
			\definecolor{colorbrewer3}{RGB}{244,109,67}
			\definecolor{colorbrewer4}{RGB}{253,174,97}
			\definecolor{colorbrewer5}{RGB}{254,224,139}
			\definecolor{colorbrewer6}{RGB}{217,239,139}
			\definecolor{colorbrewer7}{RGB}{166,217,106}
			\definecolor{colorbrewer8}{RGB}{102,189,99}
			\definecolor{colorbrewer9}{RGB}{26,152,80}
			\definecolor{colorbrewer10}{RGB}{0,104,55}
		},
		colorbrewer values/11/.code={
			\definecolor{colorbrewer1}{RGB}{165,0,38}
			\definecolor{colorbrewer2}{RGB}{215,48,39}
			\definecolor{colorbrewer3}{RGB}{244,109,67}
			\definecolor{colorbrewer4}{RGB}{253,174,97}
			\definecolor{colorbrewer5}{RGB}{254,224,139}
			\definecolor{colorbrewer6}{RGB}{255,255,191}
			\definecolor{colorbrewer7}{RGB}{217,239,139}
			\definecolor{colorbrewer8}{RGB}{166,217,106}
			\definecolor{colorbrewer9}{RGB}{102,189,99}
			\definecolor{colorbrewer10}{RGB}{26,152,80}
			\definecolor{colorbrewer11}{RGB}{0,104,55}
		}
	},
	colorbrewer scheme/Set1/.style={
		colorbrewer values/.is choice,	
		colorbrewer values/3/.code={
			\definecolor{colorbrewer1}{RGB}{228,26,28}
			\definecolor{colorbrewer2}{RGB}{55,126,184}
			\definecolor{colorbrewer3}{RGB}{77,175,74}
		},
		colorbrewer values=3,
		colorbrewer values/4/.code={
			\definecolor{colorbrewer1}{RGB}{228,26,28}
			\definecolor{colorbrewer2}{RGB}{55,126,184}
			\definecolor{colorbrewer3}{RGB}{77,175,74}
			\definecolor{colorbrewer4}{RGB}{152,78,163}
		},
		colorbrewer values/5/.code={
			\definecolor{colorbrewer1}{RGB}{228,26,28}
			\definecolor{colorbrewer2}{RGB}{55,126,184}
			\definecolor{colorbrewer3}{RGB}{77,175,74}
			\definecolor{colorbrewer4}{RGB}{152,78,163}
			\definecolor{colorbrewer5}{RGB}{255,127,0}
		},
		colorbrewer values/6/.code={
			\definecolor{colorbrewer1}{RGB}{228,26,28}
			\definecolor{colorbrewer2}{RGB}{55,126,184}
			\definecolor{colorbrewer3}{RGB}{77,175,74}
			\definecolor{colorbrewer4}{RGB}{152,78,163}
			\definecolor{colorbrewer5}{RGB}{255,127,0}
			\definecolor{colorbrewer6}{RGB}{255,255,51}
		},
		colorbrewer values/7/.code={
			\definecolor{colorbrewer1}{RGB}{228,26,28}
			\definecolor{colorbrewer2}{RGB}{55,126,184}
			\definecolor{colorbrewer3}{RGB}{77,175,74}
			\definecolor{colorbrewer4}{RGB}{152,78,163}
			\definecolor{colorbrewer5}{RGB}{255,127,0}
			\definecolor{colorbrewer6}{RGB}{255,255,51}
			\definecolor{colorbrewer7}{RGB}{166,86,40}
		},
		colorbrewer values/8/.code={
			\definecolor{colorbrewer1}{RGB}{228,26,28}
			\definecolor{colorbrewer2}{RGB}{55,126,184}
			\definecolor{colorbrewer3}{RGB}{77,175,74}
			\definecolor{colorbrewer4}{RGB}{152,78,163}
			\definecolor{colorbrewer5}{RGB}{255,127,0}
			\definecolor{colorbrewer6}{RGB}{255,255,51}
			\definecolor{colorbrewer7}{RGB}{166,86,40}
			\definecolor{colorbrewer8}{RGB}{247,129,191}
		},
		colorbrewer values/9/.code={
			\definecolor{colorbrewer1}{RGB}{228,26,28}
			\definecolor{colorbrewer2}{RGB}{55,126,184}
			\definecolor{colorbrewer3}{RGB}{77,175,74}
			\definecolor{colorbrewer4}{RGB}{152,78,163}
			\definecolor{colorbrewer5}{RGB}{255,127,0}
			\definecolor{colorbrewer6}{RGB}{255,255,51}
			\definecolor{colorbrewer7}{RGB}{166,86,40}
			\definecolor{colorbrewer8}{RGB}{247,129,191}
			\definecolor{colorbrewer9}{RGB}{153,153,153}
		}
	},
	colorbrewer scheme/Set2/.style={
		colorbrewer values/.is choice,	
		colorbrewer values/3/.code={
			\definecolor{colorbrewer1}{RGB}{102,194,165}
			\definecolor{colorbrewer2}{RGB}{252,141,98}
			\definecolor{colorbrewer3}{RGB}{141,160,203}
		},
		colorbrewer values=3,
		colorbrewer values/4/.code={
			\definecolor{colorbrewer1}{RGB}{102,194,165}
			\definecolor{colorbrewer2}{RGB}{252,141,98}
			\definecolor{colorbrewer3}{RGB}{141,160,203}
			\definecolor{colorbrewer4}{RGB}{231,138,195}
		},
		colorbrewer values/5/.code={
			\definecolor{colorbrewer1}{RGB}{102,194,165}
			\definecolor{colorbrewer2}{RGB}{252,141,98}
			\definecolor{colorbrewer3}{RGB}{141,160,203}
			\definecolor{colorbrewer4}{RGB}{231,138,195}
			\definecolor{colorbrewer5}{RGB}{166,216,84}
		},
		colorbrewer values/6/.code={
			\definecolor{colorbrewer1}{RGB}{102,194,165}
			\definecolor{colorbrewer2}{RGB}{252,141,98}
			\definecolor{colorbrewer3}{RGB}{141,160,203}
			\definecolor{colorbrewer4}{RGB}{231,138,195}
			\definecolor{colorbrewer5}{RGB}{166,216,84}
			\definecolor{colorbrewer6}{RGB}{255,217,47}
		},
		colorbrewer values/7/.code={
			\definecolor{colorbrewer1}{RGB}{102,194,165}
			\definecolor{colorbrewer2}{RGB}{252,141,98}
			\definecolor{colorbrewer3}{RGB}{141,160,203}
			\definecolor{colorbrewer4}{RGB}{231,138,195}
			\definecolor{colorbrewer5}{RGB}{166,216,84}
			\definecolor{colorbrewer6}{RGB}{255,217,47}
			\definecolor{colorbrewer7}{RGB}{229,196,148}
		},
		colorbrewer values/8/.code={
			\definecolor{colorbrewer1}{RGB}{102,194,165}
			\definecolor{colorbrewer2}{RGB}{252,141,98}
			\definecolor{colorbrewer3}{RGB}{141,160,203}
			\definecolor{colorbrewer4}{RGB}{231,138,195}
			\definecolor{colorbrewer5}{RGB}{166,216,84}
			\definecolor{colorbrewer6}{RGB}{255,217,47}
			\definecolor{colorbrewer7}{RGB}{229,196,148}
			\definecolor{colorbrewer8}{RGB}{179,179,179}
		}
	},
	colorbrewer scheme/Set3/.style={
		colorbrewer values/.is choice,	
		colorbrewer values/3/.code={
			\definecolor{colorbrewer1}{RGB}{141,211,199}
			\definecolor{colorbrewer2}{RGB}{255,255,179}
			\definecolor{colorbrewer3}{RGB}{190,186,218}
		},
		colorbrewer values=3,
		colorbrewer values/4/.code={
			\definecolor{colorbrewer1}{RGB}{141,211,199}
			\definecolor{colorbrewer2}{RGB}{255,255,179}
			\definecolor{colorbrewer3}{RGB}{190,186,218}
			\definecolor{colorbrewer4}{RGB}{251,128,114}
		},
		colorbrewer values/5/.code={
			\definecolor{colorbrewer1}{RGB}{141,211,199}
			\definecolor{colorbrewer2}{RGB}{255,255,179}
			\definecolor{colorbrewer3}{RGB}{190,186,218}
			\definecolor{colorbrewer4}{RGB}{251,128,114}
			\definecolor{colorbrewer5}{RGB}{128,177,211}
		},
		colorbrewer values/6/.code={
			\definecolor{colorbrewer1}{RGB}{141,211,199}
			\definecolor{colorbrewer2}{RGB}{255,255,179}
			\definecolor{colorbrewer3}{RGB}{190,186,218}
			\definecolor{colorbrewer4}{RGB}{251,128,114}
			\definecolor{colorbrewer5}{RGB}{128,177,211}
			\definecolor{colorbrewer6}{RGB}{253,180,98}
		},
		colorbrewer values/7/.code={
			\definecolor{colorbrewer1}{RGB}{141,211,199}
			\definecolor{colorbrewer2}{RGB}{255,255,179}
			\definecolor{colorbrewer3}{RGB}{190,186,218}
			\definecolor{colorbrewer4}{RGB}{251,128,114}
			\definecolor{colorbrewer5}{RGB}{128,177,211}
			\definecolor{colorbrewer6}{RGB}{253,180,98}
			\definecolor{colorbrewer7}{RGB}{179,222,105}
		},
		colorbrewer values/8/.code={
			\definecolor{colorbrewer1}{RGB}{141,211,199}
			\definecolor{colorbrewer2}{RGB}{255,255,179}
			\definecolor{colorbrewer3}{RGB}{190,186,218}
			\definecolor{colorbrewer4}{RGB}{251,128,114}
			\definecolor{colorbrewer5}{RGB}{128,177,211}
			\definecolor{colorbrewer6}{RGB}{253,180,98}
			\definecolor{colorbrewer7}{RGB}{179,222,105}
			\definecolor{colorbrewer8}{RGB}{252,205,229}
		},
		colorbrewer values/9/.code={
			\definecolor{colorbrewer1}{RGB}{141,211,199}
			\definecolor{colorbrewer2}{RGB}{255,255,179}
			\definecolor{colorbrewer3}{RGB}{190,186,218}
			\definecolor{colorbrewer4}{RGB}{251,128,114}
			\definecolor{colorbrewer5}{RGB}{128,177,211}
			\definecolor{colorbrewer6}{RGB}{253,180,98}
			\definecolor{colorbrewer7}{RGB}{179,222,105}
			\definecolor{colorbrewer8}{RGB}{252,205,229}
			\definecolor{colorbrewer9}{RGB}{217,217,217}
		},
		colorbrewer values/10/.code={
			\definecolor{colorbrewer1}{RGB}{141,211,199}
			\definecolor{colorbrewer2}{RGB}{255,255,179}
			\definecolor{colorbrewer3}{RGB}{190,186,218}
			\definecolor{colorbrewer4}{RGB}{251,128,114}
			\definecolor{colorbrewer5}{RGB}{128,177,211}
			\definecolor{colorbrewer6}{RGB}{253,180,98}
			\definecolor{colorbrewer7}{RGB}{179,222,105}
			\definecolor{colorbrewer8}{RGB}{252,205,229}
			\definecolor{colorbrewer9}{RGB}{217,217,217}
			\definecolor{colorbrewer10}{RGB}{188,128,189}
		},
		colorbrewer values/11/.code={
			\definecolor{colorbrewer1}{RGB}{141,211,199}
			\definecolor{colorbrewer2}{RGB}{255,255,179}
			\definecolor{colorbrewer3}{RGB}{190,186,218}
			\definecolor{colorbrewer4}{RGB}{251,128,114}
			\definecolor{colorbrewer5}{RGB}{128,177,211}
			\definecolor{colorbrewer6}{RGB}{253,180,98}
			\definecolor{colorbrewer7}{RGB}{179,222,105}
			\definecolor{colorbrewer8}{RGB}{252,205,229}
			\definecolor{colorbrewer9}{RGB}{217,217,217}
			\definecolor{colorbrewer10}{RGB}{188,128,189}
			\definecolor{colorbrewer11}{RGB}{204,235,197}
		},
		colorbrewer values/12/.code={
			\definecolor{colorbrewer1}{RGB}{141,211,199}
			\definecolor{colorbrewer2}{RGB}{255,255,179}
			\definecolor{colorbrewer3}{RGB}{190,186,218}
			\definecolor{colorbrewer4}{RGB}{251,128,114}
			\definecolor{colorbrewer5}{RGB}{128,177,211}
			\definecolor{colorbrewer6}{RGB}{253,180,98}
			\definecolor{colorbrewer7}{RGB}{179,222,105}
			\definecolor{colorbrewer8}{RGB}{252,205,229}
			\definecolor{colorbrewer9}{RGB}{217,217,217}
			\definecolor{colorbrewer10}{RGB}{188,128,189}
			\definecolor{colorbrewer11}{RGB}{204,235,197}
			\definecolor{colorbrewer12}{RGB}{255,237,111}
		}
	},
	colorbrewer scheme/Spectral/.style={
		colorbrewer values/.is choice,	
		colorbrewer values/3/.code={
			\definecolor{colorbrewer1}{RGB}{252,141,89}
			\definecolor{colorbrewer2}{RGB}{255,255,191}
			\definecolor{colorbrewer3}{RGB}{153,213,148}
		},
		colorbrewer values=3,
		colorbrewer values/4/.code={
			\definecolor{colorbrewer1}{RGB}{215,25,28}
			\definecolor{colorbrewer2}{RGB}{253,174,97}
			\definecolor{colorbrewer3}{RGB}{171,221,164}
			\definecolor{colorbrewer4}{RGB}{43,131,186}
		},
		colorbrewer values/5/.code={
			\definecolor{colorbrewer1}{RGB}{215,25,28}
			\definecolor{colorbrewer2}{RGB}{253,174,97}
			\definecolor{colorbrewer3}{RGB}{255,255,191}
			\definecolor{colorbrewer4}{RGB}{171,221,164}
			\definecolor{colorbrewer5}{RGB}{43,131,186}
		},
		colorbrewer values/6/.code={
			\definecolor{colorbrewer1}{RGB}{213,62,79}
			\definecolor{colorbrewer2}{RGB}{252,141,89}
			\definecolor{colorbrewer3}{RGB}{254,224,139}
			\definecolor{colorbrewer4}{RGB}{230,245,152}
			\definecolor{colorbrewer5}{RGB}{153,213,148}
			\definecolor{colorbrewer6}{RGB}{50,136,189}
		},
		colorbrewer values/7/.code={
			\definecolor{colorbrewer1}{RGB}{213,62,79}
			\definecolor{colorbrewer2}{RGB}{252,141,89}
			\definecolor{colorbrewer3}{RGB}{254,224,139}
			\definecolor{colorbrewer4}{RGB}{255,255,191}
			\definecolor{colorbrewer5}{RGB}{230,245,152}
			\definecolor{colorbrewer6}{RGB}{153,213,148}
			\definecolor{colorbrewer7}{RGB}{50,136,189}
		},
		colorbrewer values/8/.code={
			\definecolor{colorbrewer1}{RGB}{213,62,79}
			\definecolor{colorbrewer2}{RGB}{244,109,67}
			\definecolor{colorbrewer3}{RGB}{253,174,97}
			\definecolor{colorbrewer4}{RGB}{254,224,139}
			\definecolor{colorbrewer5}{RGB}{230,245,152}
			\definecolor{colorbrewer6}{RGB}{171,221,164}
			\definecolor{colorbrewer7}{RGB}{102,194,165}
			\definecolor{colorbrewer8}{RGB}{50,136,189}
		},
		colorbrewer values/9/.code={
			\definecolor{colorbrewer1}{RGB}{213,62,79}
			\definecolor{colorbrewer2}{RGB}{244,109,67}
			\definecolor{colorbrewer3}{RGB}{253,174,97}
			\definecolor{colorbrewer4}{RGB}{254,224,139}
			\definecolor{colorbrewer5}{RGB}{255,255,191}
			\definecolor{colorbrewer6}{RGB}{230,245,152}
			\definecolor{colorbrewer7}{RGB}{171,221,164}
			\definecolor{colorbrewer8}{RGB}{102,194,165}
			\definecolor{colorbrewer9}{RGB}{50,136,189}
		},
		colorbrewer values/10/.code={
			\definecolor{colorbrewer1}{RGB}{158,1,66}
			\definecolor{colorbrewer2}{RGB}{213,62,79}
			\definecolor{colorbrewer3}{RGB}{244,109,67}
			\definecolor{colorbrewer4}{RGB}{253,174,97}
			\definecolor{colorbrewer5}{RGB}{254,224,139}
			\definecolor{colorbrewer6}{RGB}{230,245,152}
			\definecolor{colorbrewer7}{RGB}{171,221,164}
			\definecolor{colorbrewer8}{RGB}{102,194,165}
			\definecolor{colorbrewer9}{RGB}{50,136,189}
			\definecolor{colorbrewer10}{RGB}{94,79,162}
		},
		colorbrewer values/11/.code={
			\definecolor{colorbrewer1}{RGB}{158,1,66}
			\definecolor{colorbrewer2}{RGB}{213,62,79}
			\definecolor{colorbrewer3}{RGB}{244,109,67}
			\definecolor{colorbrewer4}{RGB}{253,174,97}
			\definecolor{colorbrewer5}{RGB}{254,224,139}
			\definecolor{colorbrewer6}{RGB}{255,255,191}
			\definecolor{colorbrewer7}{RGB}{230,245,152}
			\definecolor{colorbrewer8}{RGB}{171,221,164}
			\definecolor{colorbrewer9}{RGB}{102,194,165}
			\definecolor{colorbrewer10}{RGB}{50,136,189}
			\definecolor{colorbrewer11}{RGB}{94,79,162}
		}
	},
	colorbrewer scheme/YlGn/.style={
		colorbrewer values/.is choice,	
		colorbrewer values/3/.code={
			\definecolor{colorbrewer1}{RGB}{247,252,185}
			\definecolor{colorbrewer2}{RGB}{173,221,142}
			\definecolor{colorbrewer3}{RGB}{49,163,84}
		},
		colorbrewer values=3,
		colorbrewer values/4/.code={
			\definecolor{colorbrewer1}{RGB}{255,255,204}
			\definecolor{colorbrewer2}{RGB}{194,230,153}
			\definecolor{colorbrewer3}{RGB}{120,198,121}
			\definecolor{colorbrewer4}{RGB}{35,132,67}
		},
		colorbrewer values/5/.code={
			\definecolor{colorbrewer1}{RGB}{255,255,204}
			\definecolor{colorbrewer2}{RGB}{194,230,153}
			\definecolor{colorbrewer3}{RGB}{120,198,121}
			\definecolor{colorbrewer4}{RGB}{49,163,84}
			\definecolor{colorbrewer5}{RGB}{0,104,55}
		},
		colorbrewer values/6/.code={
			\definecolor{colorbrewer1}{RGB}{255,255,204}
			\definecolor{colorbrewer2}{RGB}{217,240,163}
			\definecolor{colorbrewer3}{RGB}{173,221,142}
			\definecolor{colorbrewer4}{RGB}{120,198,121}
			\definecolor{colorbrewer5}{RGB}{49,163,84}
			\definecolor{colorbrewer6}{RGB}{0,104,55}
		},
		colorbrewer values/7/.code={
			\definecolor{colorbrewer1}{RGB}{255,255,204}
			\definecolor{colorbrewer2}{RGB}{217,240,163}
			\definecolor{colorbrewer3}{RGB}{173,221,142}
			\definecolor{colorbrewer4}{RGB}{120,198,121}
			\definecolor{colorbrewer5}{RGB}{65,171,93}
			\definecolor{colorbrewer6}{RGB}{35,132,67}
			\definecolor{colorbrewer7}{RGB}{0,90,50}
		},
		colorbrewer values/8/.code={
			\definecolor{colorbrewer1}{RGB}{255,255,229}
			\definecolor{colorbrewer2}{RGB}{247,252,185}
			\definecolor{colorbrewer3}{RGB}{217,240,163}
			\definecolor{colorbrewer4}{RGB}{173,221,142}
			\definecolor{colorbrewer5}{RGB}{120,198,121}
			\definecolor{colorbrewer6}{RGB}{65,171,93}
			\definecolor{colorbrewer7}{RGB}{35,132,67}
			\definecolor{colorbrewer8}{RGB}{0,90,50}
		},
		colorbrewer values/9/.code={
			\definecolor{colorbrewer1}{RGB}{255,255,229}
			\definecolor{colorbrewer2}{RGB}{247,252,185}
			\definecolor{colorbrewer3}{RGB}{217,240,163}
			\definecolor{colorbrewer4}{RGB}{173,221,142}
			\definecolor{colorbrewer5}{RGB}{120,198,121}
			\definecolor{colorbrewer6}{RGB}{65,171,93}
			\definecolor{colorbrewer7}{RGB}{35,132,67}
			\definecolor{colorbrewer8}{RGB}{0,104,55}
			\definecolor{colorbrewer9}{RGB}{0,69,41}
		}
	},
	colorbrewer scheme/YlGnBu/.style={
		colorbrewer values/.is choice,	
		colorbrewer values/3/.code={
			\definecolor{colorbrewer1}{RGB}{237,248,177}
			\definecolor{colorbrewer2}{RGB}{127,205,187}
			\definecolor{colorbrewer3}{RGB}{44,127,184}
		},
		colorbrewer values=3,
		colorbrewer values/4/.code={
			\definecolor{colorbrewer1}{RGB}{255,255,204}
			\definecolor{colorbrewer2}{RGB}{161,218,180}
			\definecolor{colorbrewer3}{RGB}{65,182,196}
			\definecolor{colorbrewer4}{RGB}{34,94,168}
		},
		colorbrewer values/5/.code={
			\definecolor{colorbrewer1}{RGB}{255,255,204}
			\definecolor{colorbrewer2}{RGB}{161,218,180}
			\definecolor{colorbrewer3}{RGB}{65,182,196}
			\definecolor{colorbrewer4}{RGB}{44,127,184}
			\definecolor{colorbrewer5}{RGB}{37,52,148}
		},
		colorbrewer values/6/.code={
			\definecolor{colorbrewer1}{RGB}{255,255,204}
			\definecolor{colorbrewer2}{RGB}{199,233,180}
			\definecolor{colorbrewer3}{RGB}{127,205,187}
			\definecolor{colorbrewer4}{RGB}{65,182,196}
			\definecolor{colorbrewer5}{RGB}{44,127,184}
			\definecolor{colorbrewer6}{RGB}{37,52,148}
		},
		colorbrewer values/7/.code={
			\definecolor{colorbrewer1}{RGB}{255,255,204}
			\definecolor{colorbrewer2}{RGB}{199,233,180}
			\definecolor{colorbrewer3}{RGB}{127,205,187}
			\definecolor{colorbrewer4}{RGB}{65,182,196}
			\definecolor{colorbrewer5}{RGB}{29,145,192}
			\definecolor{colorbrewer6}{RGB}{34,94,168}
			\definecolor{colorbrewer7}{RGB}{12,44,132}
		},
		colorbrewer values/8/.code={
			\definecolor{colorbrewer1}{RGB}{255,255,217}
			\definecolor{colorbrewer2}{RGB}{237,248,177}
			\definecolor{colorbrewer3}{RGB}{199,233,180}
			\definecolor{colorbrewer4}{RGB}{127,205,187}
			\definecolor{colorbrewer5}{RGB}{65,182,196}
			\definecolor{colorbrewer6}{RGB}{29,145,192}
			\definecolor{colorbrewer7}{RGB}{34,94,168}
			\definecolor{colorbrewer8}{RGB}{12,44,132}
		},
		colorbrewer values/9/.code={
			\definecolor{colorbrewer1}{RGB}{255,255,217}
			\definecolor{colorbrewer2}{RGB}{237,248,177}
			\definecolor{colorbrewer3}{RGB}{199,233,180}
			\definecolor{colorbrewer4}{RGB}{127,205,187}
			\definecolor{colorbrewer5}{RGB}{65,182,196}
			\definecolor{colorbrewer6}{RGB}{29,145,192}
			\definecolor{colorbrewer7}{RGB}{34,94,168}
			\definecolor{colorbrewer8}{RGB}{37,52,148}
			\definecolor{colorbrewer9}{RGB}{8,29,88}
		}
	},
	colorbrewer scheme/YlOrBr/.style={
		colorbrewer values/.is choice,	
		colorbrewer values/3/.code={
			\definecolor{colorbrewer1}{RGB}{255,247,188}
			\definecolor{colorbrewer2}{RGB}{254,196,79}
			\definecolor{colorbrewer3}{RGB}{217,95,14}
		},
		colorbrewer values=3,
		colorbrewer values/4/.code={
			\definecolor{colorbrewer1}{RGB}{255,255,212}
			\definecolor{colorbrewer2}{RGB}{254,217,142}
			\definecolor{colorbrewer3}{RGB}{254,153,41}
			\definecolor{colorbrewer4}{RGB}{204,76,2}
		},
		colorbrewer values/5/.code={
			\definecolor{colorbrewer1}{RGB}{255,255,212}
			\definecolor{colorbrewer2}{RGB}{254,217,142}
			\definecolor{colorbrewer3}{RGB}{254,153,41}
			\definecolor{colorbrewer4}{RGB}{217,95,14}
			\definecolor{colorbrewer5}{RGB}{153,52,4}
		},
		colorbrewer values/6/.code={
			\definecolor{colorbrewer1}{RGB}{255,255,212}
			\definecolor{colorbrewer2}{RGB}{254,227,145}
			\definecolor{colorbrewer3}{RGB}{254,196,79}
			\definecolor{colorbrewer4}{RGB}{254,153,41}
			\definecolor{colorbrewer5}{RGB}{217,95,14}
			\definecolor{colorbrewer6}{RGB}{153,52,4}
		},
		colorbrewer values/7/.code={
			\definecolor{colorbrewer1}{RGB}{255,255,212}
			\definecolor{colorbrewer2}{RGB}{254,227,145}
			\definecolor{colorbrewer3}{RGB}{254,196,79}
			\definecolor{colorbrewer4}{RGB}{254,153,41}
			\definecolor{colorbrewer5}{RGB}{236,112,20}
			\definecolor{colorbrewer6}{RGB}{204,76,2}
			\definecolor{colorbrewer7}{RGB}{140,45,4}
		},
		colorbrewer values/8/.code={
			\definecolor{colorbrewer1}{RGB}{255,255,229}
			\definecolor{colorbrewer2}{RGB}{255,247,188}
			\definecolor{colorbrewer3}{RGB}{254,227,145}
			\definecolor{colorbrewer4}{RGB}{254,196,79}
			\definecolor{colorbrewer5}{RGB}{254,153,41}
			\definecolor{colorbrewer6}{RGB}{236,112,20}
			\definecolor{colorbrewer7}{RGB}{204,76,2}
			\definecolor{colorbrewer8}{RGB}{140,45,4}
		},
		colorbrewer values/9/.code={
			\definecolor{colorbrewer1}{RGB}{255,255,229}
			\definecolor{colorbrewer2}{RGB}{255,247,188}
			\definecolor{colorbrewer3}{RGB}{254,227,145}
			\definecolor{colorbrewer4}{RGB}{254,196,79}
			\definecolor{colorbrewer5}{RGB}{254,153,41}
			\definecolor{colorbrewer6}{RGB}{236,112,20}
			\definecolor{colorbrewer7}{RGB}{204,76,2}
			\definecolor{colorbrewer8}{RGB}{153,52,4}
			\definecolor{colorbrewer9}{RGB}{102,37,6}
		}
	},
	colorbrewer scheme/YlOrRd/.style={
		colorbrewer values/.is choice,	
		colorbrewer values/3/.code={
			\definecolor{colorbrewer1}{RGB}{255,237,160}
			\definecolor{colorbrewer2}{RGB}{254,178,76}
			\definecolor{colorbrewer3}{RGB}{240,59,32}
		},
		colorbrewer values=3,
		colorbrewer values/4/.code={
			\definecolor{colorbrewer1}{RGB}{255,255,178}
			\definecolor{colorbrewer2}{RGB}{254,204,92}
			\definecolor{colorbrewer3}{RGB}{253,141,60}
			\definecolor{colorbrewer4}{RGB}{227,26,28}
		},
		colorbrewer values/5/.code={
			\definecolor{colorbrewer1}{RGB}{255,255,178}
			\definecolor{colorbrewer2}{RGB}{254,204,92}
			\definecolor{colorbrewer3}{RGB}{253,141,60}
			\definecolor{colorbrewer4}{RGB}{240,59,32}
			\definecolor{colorbrewer5}{RGB}{189,0,38}
		},
		colorbrewer values/6/.code={
			\definecolor{colorbrewer1}{RGB}{255,255,178}
			\definecolor{colorbrewer2}{RGB}{254,217,118}
			\definecolor{colorbrewer3}{RGB}{254,178,76}
			\definecolor{colorbrewer4}{RGB}{253,141,60}
			\definecolor{colorbrewer5}{RGB}{240,59,32}
			\definecolor{colorbrewer6}{RGB}{189,0,38}
		},
		colorbrewer values/7/.code={
			\definecolor{colorbrewer1}{RGB}{255,255,178}
			\definecolor{colorbrewer2}{RGB}{254,217,118}
			\definecolor{colorbrewer3}{RGB}{254,178,76}
			\definecolor{colorbrewer4}{RGB}{253,141,60}
			\definecolor{colorbrewer5}{RGB}{252,78,42}
			\definecolor{colorbrewer6}{RGB}{227,26,28}
			\definecolor{colorbrewer7}{RGB}{177,0,38}
		},
		colorbrewer values/8/.code={
			\definecolor{colorbrewer1}{RGB}{255,255,204}
			\definecolor{colorbrewer2}{RGB}{255,237,160}
			\definecolor{colorbrewer3}{RGB}{254,217,118}
			\definecolor{colorbrewer4}{RGB}{254,178,76}
			\definecolor{colorbrewer5}{RGB}{253,141,60}
			\definecolor{colorbrewer6}{RGB}{252,78,42}
			\definecolor{colorbrewer7}{RGB}{227,26,28}
			\definecolor{colorbrewer8}{RGB}{177,0,38}
		},
		colorbrewer values/9/.code={
			\definecolor{colorbrewer1}{RGB}{255,255,204}
			\definecolor{colorbrewer2}{RGB}{255,237,160}
			\definecolor{colorbrewer3}{RGB}{254,217,118}
			\definecolor{colorbrewer4}{RGB}{254,178,76}
			\definecolor{colorbrewer5}{RGB}{253,141,60}
			\definecolor{colorbrewer6}{RGB}{252,78,42}
			\definecolor{colorbrewer7}{RGB}{227,26,28}
			\definecolor{colorbrewer8}{RGB}{189,0,38}
			\definecolor{colorbrewer9}{RGB}{128,0,38}
		}
	}
}
