# Supplementary material for: Blind Image Restoration with Flow Based Priors
Source: arXiv:2009.04583 source file (2020-09-09)
Supplement: Supplementary file 4 [file includes.tex]

%\makeatletter
%\@namedef{ver@everyshi.sty}{}
%\makeatother
%\usepackage{tikz}
%\usepackage{epstopdf}
%\usepackage{subfig}
%\usepackage{makecell}
%\usepackage{booktabs}
%\usepackage{algpseudocode}
%\usepackage{algorithm}

% references and abbreviations
\newcommand{\refsec}[1]{Section~\ref{#1}}
\newcommand{\refsecb}[1]{Sec.~\ref{#1}}
\newcommand{\refch}[1]{Chapter~\ref{#1}}
%\newcommand{\refeq}[1]{Equation~\eqref{#1}}
\newcommand{\refeqb}[1]{Eq.~\ref{#1}}
\newcommand{\reffig}[1]{Figure~\ref{#1}}
\newcommand{\reffigb}[1]{Fig.~\ref{#1}}
\newcommand{\reftab}[1]{Table~\ref{#1}}
\newcommand{\refalg}[1]{Algorithm~\ref{#1}}
\newcommand{\var}[1]{\text{#1}}

%\usepackage[bottom]{footmisc}

% comments
%\definecolor{myred}{RGB}{200,100,0}
%\definecolor{myblue}{RGB}{10,10,200}
%\definecolor{mygreen}{RGB}{10,150,100}
%\definecolor{myorange}{RGB}{255,165,0}
%
%\newcommand{\cpFire}[0]{\copyright~Vision Research~\cite{VR}}
%\newcommand{\cpWater}[0]{\copyright~Vision Research~\cite{VR}}
%\newcommand{\cpBlender}[0]{\copyright~Blender Foundation~\cite{Blender}}
%
%
%
%\newcommand{\sm}[1]{{\color{myblue}\textbf{[SM: }\textit{#1}\textbf{]}}}
%% %% REMOVE ALL COMMENTS
%%\renewcommand{\sm}[1]{}
%
%\DeclareMathOperator*{\argmin}{arg\,min}
%
%\newcommand{\atan}{\mathrm{atan2}}
%
%\makeatletter
%\renewcommand{\paragraph}{%
%	\@startsection{paragraph}{4}%
%	{\z@}{1.25ex \@plus 1ex \@minus .2ex}{-1em}%
%	{\normalfont\normalsize\bfseries}%
%}
%\makeatother
%
%%%%%%%%%%%%%%%%%%%%%%%%%%%%%%%%%%%%%%%%%%%%%%%%%%%%%%%%%%%%%%%%%%%%%%%%%%
%%%%%%%%%%%%%%%%%%%%%%%%%%%%%%%%%%%%%%%%%%%%%%%%%%%%%%%%%%%%%%%%%%%%%%%%%%
%%  Set the following to 0 to include full-size images and only trim them
%%  Set it to 1 to include cropped images
%\gdef\useCroppedImages{1}
%
%%  Set to 1 to (re)create cropped images for all figures
%%  Make sure to compile with --shell-escape (e.g. pdflatex --shell-escape paper.tex)
%\gdef\cropInsets{1}
%%%%%%%%%%%%%%%%%%%%%%%%%%%%%%%%%%%%%%%%%%%%%%%%%%%%%%%%%%%%%%%%%%%%%%%%%%
%
%\usepackage[export]{adjustbox}
%\usepackage{calc}
%\usepackage{tabularx}
%\usepackage{tikz}
%\usepackage{xstring}
%\usepackage{float}
%
%\renewcommand{\fboxsep}{0pt}
%\newcommand{\cfbox}[2]{%
%	\colorlet{currentcolor}{.}%
%	{\color{#1}%
%		\fbox{\color{currentcolor}#2}}%
%}
%\newcommand{\cframebox}[4]{%
%	\linethickness{1pt}
%	\colorlet{currentcolor}{.}%
%	{\color{#3}%
%		\framebox(#1,#2){\color{currentcolor}#4}}%
%}
%
%\newlength\beautyHeight
%\newlength\beautyPixWidth
%\newlength\beautyPixHeight
%% Vertical separation between insets
%\newlength\insetvsep
%\setlength\insetvsep{0pt}
%% Variables for enabling insets and setting the crop region
%\gdef\useInsetA{0}
%\gdef\useInsetB{0}
%\gdef\useInsetC{0}
%
%\newcommand{\setInset}[6]{%
%	\expandafter\gdef\csname useInset#1\endcsname{1}%
%	\expandafter\gdef\csname inset#1Color\endcsname{#2}%
%	\expandafter\gdef\csname crop#1X\endcsname{#3}%
%	\expandafter\gdef\csname crop#1Y\endcsname{#4}%
%	\expandafter\gdef\csname crop#1W\endcsname{#5}%
%	\expandafter\gdef\csname crop#1H\endcsname{#6}%
%}
%
%\newcommand{\unsetInset}[1]{%
%	\expandafter\gdef\csname useInset#1\endcsname{0}%
%}
%
%\newcommand{\addBeautyCrop}[8]{%
%	% #1 - filename
%	% #2 - width as \textwidth multiple
%	% #3 - pixel width
%	% #4 - pixel height
%	% #5 - crop X pixel pos
%	% #6 - crop Y pixel pos
%	% #7 - crop width in pixels
%	% #8 - crop height in pixels
%	\pdfpxdimen=\dimexpr 1 in/72\relax
%	\def\beauty{%
%		\let\cropR\relax%
%		\let\cropB\relax%
%		\newlength\cropR%
%		\newlength\cropB%
%		\setlength\cropR{{#3 px}-{#5 px}-{#7 px}}%
%		\setlength\cropB{{#4 px}-{#6 px}-{#8 px}}%
%		\sbox0{\includegraphics[width=#2\textwidth,trim={#5px {\cropB} {\cropR} #6px},clip]{#1}}%
%		\begin{tikzpicture}
%		\node[anchor=north west,inner sep=0] at (0,0) {\usebox0};
%		\begin{scope}[x=\wd0/#7, y=\ht0/#8]
%		\if\useInsetA1{
%			\draw[\insetAColor,thick] (\cropAX-#5,-\cropAY+#6) rectangle + (\cropAW,-\cropAH);
%		}\fi
%		\if\useInsetB1{
%			\draw[\insetBColor,thick] (\cropBX-#5,-\cropBY+#6) rectangle + (\cropBW,-\cropBH);
%		}\fi
%		\if\useInsetC1{
%			\draw[\insetCColor,thick] (\cropCX-#5,-\cropCY+#6) rectangle + (\cropCW,-\cropCH);
%		}\fi
%		\end{scope}
%		\end{tikzpicture}
%	}%
%	\setlength\beautyHeight{\heightof{\beauty}}%
%	\setlength\beautyPixWidth{#3px}%
%	\setlength\beautyPixHeight{#4px}%
%	\global\beautyHeight=\beautyHeight%
%	\global\beautyPixWidth=\beautyPixWidth%
%	\global\beautyPixHeight=\beautyPixHeight%
%	\begin{adjustbox}{valign=t}
%		\beauty
%	\end{adjustbox}
%}
%
%\newcommand{\addBeauty}[4]{%
%	\addBeautyCrop{#1}{#2}{#3}{#4}{0}{0}{#3}{#4}%
%}
%
%% \newcommand{\setBeautyCrop}[8]{%
%%     % #1 - filename
%%     % #2 - width as \textwidth multiple
%%     % #3 - pixel width
%%     % #4 - pixel height
%%     % #5 - crop X pixel pos
%%     % #6 - crop Y pixel pos
%%     % #7 - crop width in pixels
%%     % #8 - crop height in pixels
%%     \pdfpxdimen=\dimexpr 1 in/72\relax
%%     \def\beauty{%
%%         \let\cropR\relax%
%%         \let\cropB\relax%
%%         \newlength\cropR%
%%         \newlength\cropB%
%%         \setlength\cropR{{#3 px}-{#5 px}-{#7 px}}%
%%         \setlength\cropB{{#4 px}-{#6 px}-{#8 px}}%
%%     }%
%%     \setlength\beautyHeight{#8px}%\heightof{\beauty}}%
%%     \setlength\beautyPixWidth{#3px}%
%%     \setlength\beautyPixHeight{#4px}%
%%     \global\beautyHeight=\beautyHeight%
%%     \global\beautyPixWidth=\beautyPixWidth%
%%     \global\beautyPixHeight=\beautyPixHeight%
%%     \begin{adjustbox}{valign=t}
%%         \beauty
%%     \end{adjustbox}
%% }
%
%% \newcommand{\setBeauty}[4]{%
%%     \setBeautyCrop{#1}{#2}{#3}{#4}{0}{0}{#3}{#4}%
%% }
%
%\newcommand{\trimInset}[6]{%
%	\let\cropR\relax%
%	\let\cropB\relax%
%	\newlength\cropR%
%	\newlength\cropB%
%	\setlength\cropR{{\beautyPixWidth}-{#3 px}-{#5 px}}%
%	\setlength\cropB{{\beautyPixHeight}-{#4 px}-{#6 px}}%
%	\color{#2}%
%	\fbox{\includegraphics[width=1\linewidth,trim={{#3 px} {\cropB} {\cropR} {#4 px}},clip]{#1}}%
%}
%
%\newcommand{\addInset}[2]{%
%	\color{#2}%
%	\fbox{\includegraphics[width=1\linewidth]{#1}}%
%}
%
%\newcommand{\auxtimes}{x}
%\newcommand{\auxplus}{+}
%\newcommand{\auxspace}{ }
%
%\newcommand{\addInsets}[2][1]{%
%	\begin{adjustbox}{valign=t}
%		\StrSubstitute{#2}{.}{-}[\baseFileName]
%		\begin{adjustbox}{totalheight=#1\beautyHeight,tabular={c}}
%			\if\useInsetA1%
%			\def\cropfile{\baseFileName-\cropAW\auxtimes\cropAH\auxplus\cropAX\auxplus\cropAY}
%			\if\cropInsets1
%			\immediate\write18{convert #2 +repage -crop \cropAW\auxtimes\cropAH\auxplus\cropAX\auxplus\cropAY\auxspace \cropfile.png}
%			\fi
%			\if\useCroppedImages1
%			\addInset{\cropfile.png}{\insetAColor}
%			\else
%			\trimInset{#2}{\insetAColor}{\cropAX}{\cropAY}{\cropAW}{\cropAH}%
%			\fi%
%			\fi%
%			\if\useInsetB1%
%			\if\useInsetA1\\[\insetvsep]\fi%
%			\def\cropfile{\baseFileName-\cropBW\auxtimes\cropBH\auxplus\cropBX\auxplus\cropBY}
%			\if\cropInsets1
%			\immediate\write18{convert #2 -crop \cropBW\auxtimes\cropBH\auxplus\cropBX\auxplus\cropBY\auxspace \cropfile.png}
%			\fi
%			\if\useCroppedImages1
%			\addInset{\cropfile.png}{\insetBColor}
%			\else
%			\trimInset{#2}{\insetBColor}{\cropBX}{\cropBY}{\cropBW}{\cropBH}%
%			\fi%
%			\fi%
%			\if\useInsetC1%
%			\if\useInsetB1\\[\insetvsep]\fi%
%			\def\cropfile{\baseFileName-\cropCW\auxtimes\cropCH\auxplus\cropCX\auxplus\cropCY}
%			\if\cropInsets1
%			\immediate\write18{convert #2 -crop \cropCW\auxtimes\cropCH\auxplus\cropCX\auxplus\cropCY\auxspace \cropfile.png}
%			\fi
%			\if\useCroppedImages1
%			\addInset{\cropfile.png}{\insetCColor}
%			\else
%			\trimInset{#2}{\insetCColor}{\cropCX}{\cropCY}{\cropCW}{\cropCH}%
%			\fi%
%			\fi%
%		\end{adjustbox}
%	\end{adjustbox}
%}
%
%\newcommand{\addHorInsets}[2][1]{%
%	\begin{adjustbox}{valign=t}
%		\StrSubstitute{#2}{.}{-}[\baseFileName]
%		\begin{adjustbox}{totalheight=#1\beautyHeight,tabular={c}}
%			\if\useInsetA1%
%			\def\cropfile{\baseFileName-\cropAW\auxtimes\cropAH\auxplus\cropAX\auxplus\cropAY}
%			\if\cropInsets1
%			\immediate\write18{convert #2 -crop \cropAW\auxtimes\cropAH\auxplus\cropAX\auxplus\cropAY\auxspace \cropfile.png}
%			\fi
%			\if\useCroppedImages1
%			\addInset{\cropfile.png}{\insetAColor}
%			\else
%			\trimInset{#2}{\insetAColor}{\cropAX}{\cropAY}{\cropAW}{\cropAH}%
%			\fi%
%			\fi%
%			\if\useInsetB1%
%			%			\if\useInsetA1\\[\insetvsep]\fi%
%			\def\cropfile{\baseFileName-\cropBW\auxtimes\cropBH\auxplus\cropBX\auxplus\cropBY}
%			\if\cropInsets1
%			\immediate\write18{convert #2 -crop \cropBW\auxtimes\cropBH\auxplus\cropBX\auxplus\cropBY\auxspace \cropfile.png}
%			\fi
%			\if\useCroppedImages1
%			\addInset{\cropfile.png}{\insetBColor}
%			\else
%			\trimInset{#2}{\insetBColor}{\cropBX}{\cropBY}{\cropBW}{\cropBH}%
%			\fi%
%			\fi%
%			\if\useInsetC1%
%			%			\if\useInsetB1\\[\insetvsep]\fi%
%			\def\cropfile{\baseFileName-\cropCW\auxtimes\cropCH\auxplus\cropCX\auxplus\cropCY}
%			\if\cropInsets1
%			\immediate\write18{convert #2 -crop \cropCW\auxtimes\cropCH\auxplus\cropCX\auxplus\cropCY\auxspace \cropfile.png}
%			\fi
%			\if\useCroppedImages1
%			\addInset{\cropfile.png}{\insetCColor}
%			\else
%			\trimInset{#2}{\insetCColor}{\cropCX}{\cropCY}{\cropCW}{\cropCH}%
%			\fi%
%			\fi%
%		\end{adjustbox}
%	\end{adjustbox}
%}
%
%
%
%%%%%%%%%%%%%%%%%%%%%%%%%%%%%%%%%%%%%%%%%%%%%%%%%%%%%%%%%%%%%%%%%%%%%%%%%%
%%%%%%%%%%%%%%%%%%%%%%%%%%%%%%%%%%%%%%%%%%%%%%%%%%%%%%%%%%%%%%%%%%%%%%%%%%
%
%%%%%%%%%%%%%%%%%%%%%%%%%%%%%%%%%%%%%%%%%%%%%%%%%%%%%%%%%%%%%%%%%%%%%%
%\pgfkeys{/tikz/.cd,
%	zoombox paths/.style={
%		draw=orange,
%		very thick
%	},
%	black and white/.is choice,
%	black and white/.default=static,
%	black and white/static/.style={ 
%		draw=white,   
%		zoombox paths/.append style={
%			draw=white,
%			postaction={
%				draw=black,
%				loosely dashed
%			}
%		}
%	},
%	black and white/static/.code={
%		\gdef\patternnumber{1}
%	},
%	black and white/cycle/.code={
%		\blackandwhitecycletrue
%		\gdef\patternnumber{1}
%	},
%	black and white pattern/.is choice,
%	black and white pattern/0/.style={},
%	black and white pattern/1/.style={    
%		draw=white,
%		postaction={
%			draw=black,
%			dash pattern=on 2pt off 2pt
%		}
%	},
%	black and white pattern/2/.style={    
%		draw=white,
%		postaction={
%			draw=black,
%			dash pattern=on 4pt off 4pt
%		}
%	},
%	black and white pattern/3/.style={    
%		draw=white,
%		postaction={
%			draw=black,
%			dash pattern=on 4pt off 4pt on 1pt off 4pt
%		}
%	},
%	black and white pattern/4/.style={    
%		draw=white,
%		postaction={
%			draw=black,
%			dash pattern=on 4pt off 2pt on 2 pt off 2pt on 2 pt off 2pt
%		}
%	},
%	zoomboxarray inner gap/.initial=5pt,
%	zoomboxarray columns/.initial=2,
%	zoomboxarray rows/.initial=2,
%	subfigurename/.initial={},
%	figurename/.initial={zoombox},
%	zoomboxarray/.style={
%		execute at begin picture={
%			\begin{scope}[
%				spy using outlines={%
%					zoombox paths,
%					width=\imagewidth / \pgfkeysvalueof{/tikz/zoomboxarray columns} - (\pgfkeysvalueof{/tikz/zoomboxarray columns} - 1) / \pgfkeysvalueof{/tikz/zoomboxarray columns} * \pgfkeysvalueof{/tikz/zoomboxarray inner gap} -\pgflinewidth,
%					height=\imageheight / \pgfkeysvalueof{/tikz/zoomboxarray rows} - (\pgfkeysvalueof{/tikz/zoomboxarray rows} - 1) / \pgfkeysvalueof{/tikz/zoomboxarray rows} * \pgfkeysvalueof{/tikz/zoomboxarray inner gap}-\pgflinewidth,
%					magnification=3,
%					every spy on node/.style={
%						zoombox paths
%					},
%					every spy in node/.style={
%						zoombox paths
%					}
%				}
%				]
%			},
%			execute at end picture={
%			\end{scope}
%			\node at (image.north) [anchor=north,inner sep=0pt] {\subcaptionbox{\label{\pgfkeysvalueof{/tikz/figurename}-image}}{\phantomimage}};
%			\node at (zoomboxes container.north) [anchor=north,inner sep=0pt] {\subcaptionbox{\label{\pgfkeysvalueof{/tikz/figurename}-zoom}}{\phantomimage}};
%			\gdef\patternnumber{0}
%		},
%		spymargin/.initial=0.5em,
%		zoomboxes xshift/.initial=1,
%		zoomboxes right/.code=\pgfkeys{/tikz/zoomboxes xshift=1},
%		zoomboxes left/.code=\pgfkeys{/tikz/zoomboxes xshift=-1},
%		zoomboxes yshift/.initial=0,
%		zoomboxes above/.code={
%			\pgfkeys{/tikz/zoomboxes yshift=1},
%			\pgfkeys{/tikz/zoomboxes xshift=0}
%		},
%		zoomboxes below/.code={
%			\pgfkeys{/tikz/zoomboxes yshift=-1},
%			\pgfkeys{/tikz/zoomboxes xshift=0}
%		},
%		caption margin/.initial=4ex,
%	},
%	adjust caption spacing/.code={},
%	image container/.style={
%		inner sep=0pt,
%		at=(image.north),
%		anchor=north,
%		adjust caption spacing
%	},
%	zoomboxes container/.style={
%		inner sep=0pt,
%		at=(image.north),
%		anchor=north,
%		name=zoomboxes container,
%		xshift=\pgfkeysvalueof{/tikz/zoomboxes xshift}*(\imagewidth+\pgfkeysvalueof{/tikz/spymargin}),
%		yshift=\pgfkeysvalueof{/tikz/zoomboxes yshift}*(\imageheight+\pgfkeysvalueof{/tikz/spymargin}+\pgfkeysvalueof{/tikz/caption margin}),
%		adjust caption spacing
%	},
%	calculate dimensions/.code={
%		\pgfpointdiff{\pgfpointanchor{image}{south west} }{\pgfpointanchor{image}{north east} }
%		\pgfgetlastxy{\imagewidth}{\imageheight}
%		\global\let\imagewidth=\imagewidth
%		\global\let\imageheight=\imageheight
%		\gdef\columncount{1}
%		\gdef\rowcount{1}
%		\gdef\zoomboxcount{1}
%	},
%	image node/.style={
%		inner sep=0pt,
%		name=image,
%		anchor=south west,
%		append after command={
%			[calculate dimensions]
%			node [image container,subfigurename=\pgfkeysvalueof{/tikz/figurename}-image] {\phantomimage}
%			node [zoomboxes container,subfigurename=\pgfkeysvalueof{/tikz/figurename}-zoom] {\phantomimage}
%		}
%	},
%	color code/.style={
%		zoombox paths/.append style={draw=#1}
%	},
%	connect zoomboxes/.style={
%		spy connection path={\draw[draw=none,zoombox paths] (tikzspyonnode) -- (tikzspyinnode);}
%	},
%	help grid code/.code={
%		\begin{scope}[
%			x={(image.south east)},
%			y={(image.north west)},
%			font=\footnotesize,
%			help lines,
%			overlay
%			]
%			\foreach \x in {0,1,...,9} { 
%				\draw(\x/10,0) -- (\x/10,1);
%				\node [anchor=north] at (\x/10,0) {0.\x};
%			}
%			\foreach \y in {0,1,...,9} {
%				\draw(0,\y/10) -- (1,\y/10);                        \node [anchor=east] at (0,\y/10) {0.\y};
%			}
%		\end{scope}    
%	},
%	help grid/.style={
%		append after command={
%			[help grid code]
%		}
%	},
%}
%
%\newcommand\phantomimage{%
%	\phantom{%
%		\rule{\imagewidth}{\imageheight}%
%	}%
%}
%\newcommand\zoombox[2][]{
%	\begin{scope}[zoombox paths]
%		\pgfmathsetmacro\xpos{
%			(\columncount-1)*(\imagewidth / \pgfkeysvalueof{/tikz/zoomboxarray columns} + \pgfkeysvalueof{/tikz/zoomboxarray inner gap} / \pgfkeysvalueof{/tikz/zoomboxarray columns} ) + \pgflinewidth
%		}
%		\pgfmathsetmacro\ypos{
%			(\rowcount-1)*( \imageheight / \pgfkeysvalueof{/tikz/zoomboxarray rows} + \pgfkeysvalueof{/tikz/zoomboxarray inner gap} / \pgfkeysvalueof{/tikz/zoomboxarray rows} ) + 0.5*\pgflinewidth
%		}
%		\edef\dospy{\noexpand\spy [
%			#1,
%			zoombox paths/.append style={
%				black and white pattern=\patternnumber
%			},
%			every spy on node/.append style={#1},
%			x=\imagewidth,
%			y=\imageheight
%			] on (#2) in node [anchor=north west] at ($(zoomboxes container.north west)+(\xpos pt,-\ypos pt)$);}
%		\dospy
%		\pgfmathtruncatemacro\pgfmathresult{ifthenelse(\columncount==\pgfkeysvalueof{/tikz/zoomboxarray columns},\rowcount+1,\rowcount)}
%		\global\let\rowcount=\pgfmathresult
%		\pgfmathtruncatemacro\pgfmathresult{ifthenelse(\columncount==\pgfkeysvalueof{/tikz/zoomboxarray columns},1,\columncount+1)}
%		\global\let\columncount=\pgfmathresult
%		\ifblackandwhitecycle
%		\pgfmathtruncatemacro{\newpatternnumber}{\patternnumber+1}
%		\global\edef\patternnumber{\newpatternnumber}
%		\fi
%	\end{scope}
%}
%
%%%%%%%%%%%%%%%%%%%%%%%%%%
%\usepackage[skins]{tcolorbox} % for the teaser
%\usepackage{shadowtext}
%\shadowrgb{0,0,0}
%\shadowoffset{0.5pt}
